# Supplementary material for: Variational Inference for Stochastic Block Models from Sampled Data
Source: arXiv:1707.04141 source file (2019-01-09)
Supplement: Supplementary file 1 [file appendix_identifiability.tex]

\subsection{Identifiability}
\label{appendix:identifiability}

When the sampling is node-centered, we denote $V_i = 1$ if node $i$ is
observed and $V_i = 0$ otherwise.

\begin{proof}[Proof of
  Proposition~\ref{thm:ident_mcarParam}] %est ce claire V et R ?, changer dans les preuves les \ell en p
  Let $\rho,\rho^{\prime}>0$ be such that
  $p_\rho(R)=p_{\rho^{\prime}}(R)$
  (resp. $p_\rho(V)=p_{\rho^{\prime}}(V)$). Since $R$ (resp.$V$) does
  not depend on $\MA$, then
  $\mathbb{P}_\rho(R_{ij}=1)=\rho=\rho^{\prime}=\mathbb{P}_{\rho^{\prime}}(R_{ij}=1)$
  (resp.
  $\mathbb{P}_{\rho}(V_{i}=1)=\rho=\rho^{\prime}=\mathbb{P}_{\rho^{\prime}}(V_{i}=1)$).
\end{proof}

\begin{proof}[Proof of Theorem~\ref{thm.identifiabilityMAR}]

  Let $P_{[n]}^o$ denote the probability distribution function of
  $\Xn^o$. We show that there exists a unique $(\alpha,\pi)$
  corresponding to $P_{[n]}^o$.

  Define
  $s_q=\mathbb{P}(\MA_{ij}R_{ij}=1|Z_{iq}=1)=\rho (\pi \ \alpha )_q$
  (resp. $s_q=\mathbb{P}(\MA_{ij}=1 |Z_{iq}=1)=(\pi \ \alpha )_q$ for
  star sampling).  Up to reordering, $ s_1 < s_2 < \ldots < s_Q $ are
  the coordinates of the vector $s$ in the increasing order. Let $S$
  denote the Vandermonde matrix defined by $S_{i,q}=s_q^i$, for
  $0\leq i<Q$ and $1\leq q \leq Q$. $S$ is invertible since the
  coordinates of $s$ are all different. For $i\geq1$,
  $S_{i,q} =\mathbb{P}(\MA_{12}R_{12}=1, \ldots, \MA_{1 i+1}R_{1
    i+1}=1 | Z_{1q}=1)$ for random-dyad sampling (resp.
  $S_{i,q} =\mathbb{P}(\MA_{12}=1, \ldots, \MA_{1 i+1}=1 | Z_{1q}=1)$
  for star degree sampling).  Let us also define
  \begin{equation*}
    u_i=\sum_{1\leq k\leq Q} \alpha_k s_k^i \quad (\text{resp. $u_i=\sum_{1\leq k\leq Q} \rho \alpha_k s_k^i$}),\quad i=0,\ldots,2Q-1\enspace.
  \end{equation*}
  For $i \geq 1$,
  $u_i=\mathbb{P}(\MA_{12}R_{12}=1, \ldots, \MA_{1 i+1}R_{1 i+1}=1)$
  (resp. $u_i =\mathbb{P}(\MA_{12}=1, \ldots, \MA_{1 i+1}=1, V_1=1)$).
  Note that $n\geq 2Q$ is a necessary requirement on $n$ since
  $\MA_{i,i}=0$ by assumption.
  Hence, given $P_{[n]}^o$ and $\rho$, $u_0=1$ and
  $u_1,\ldots,u_{2Q-1}$ are known.

Furthermore, set $M$ the $(Q+1) \times Q$ matrix given by
$M_{i,j}=u_{i+j}$ for every $0\leq i\leq Q$ and $0\leq j<Q$, and
let $M_i$ denote the square matrix obtained by removing the row
$i$ from $M$. The coefficients of $M_Q$, for $0 \leq  i,j < Q$,  are
\begin{equation*}
M_{i,j}=\sum_{1\leq k \leq Q } s_k^i \alpha_k
s_k^j \quad (\text{resp. $M_{i,j}=\sum_{1\leq k \leq Q } \rho s_k^i \alpha_k
s_k^j$}) \enspace,\ \mathrm{with} \ 0 \leq  i,j < Q\enspace.
\end{equation*}

Defining the diagonal matrix $A=\mathrm{Diag}(\alpha)$, it comes
that $M_Q=SAS^{\,t}$ (resp. $M_Q=\rho SAS^{\,t}$), where $S$ and $A$ are invertible, but
unknown at this stage, and $\rho>0$.
With $D_k=\det(M_k)$ and the polynomial $B(x)=\sum_{k=0}^Q
(-1)^{k+Q} D_k\, x^k$, it yields  $D_Q=\det(M_Q)\neq0$ and the
degree of $B$ is equal to $Q$.

Set $C_i=(1,s_i,\ldots,s_i^Q)^t$ and let us notice that $B(s_i)$ is
the determinant of the square matrix produced when appending $C_i$ as
the last column to $M$.  The $Q+1$ columns of this matrix are linearly
dependent, since they are all linear combinations of the $Q$ vectors
$C_1$, $C_2$, $\ldots$, $C_Q$.  Hence $B(s_i)=0$ and $s_i$ is a root
of $B$ for every $1\leq i\leq Q$.  This proves that
$B=D_Q\prod_{i=1}^Q(x-s_i)$.  Then, one knows that
$s=(s_1,\ldots,s_Q)$ (as the roots of $B$ defined from $M$) and
$S$. It results that $A= S^{-1} M_Q (S^{\,t})^{-1}$, which yields a
unique $(\alpha_1,\ldots,\alpha_Q)$ (resp.
$A= \rho^{-1} S^{-1} M_Q (S^{\,t})^{-1}$).

It only remains to determine $\pi$. For $0 \leq i,j <Q $, let us
introduce $U_{i,j}$ the probability that the first row of $\MA^o$
begins with $i+1$ occurrences of 1, and the second row of $\MA^o$ ends
up with $j$ occurrences of 1 ($i+1+j\leq n-1$ implies $n\geq
2Q$). Then,
$U_{i,j}=\sum_{k,l} S_{i,k} \alpha_k \pi_{k,l} \alpha_l S_{j,l}$
(resp.
$U_{i,j}=\sum_{k,l} \rho^2 S_{i,k} \alpha_k \pi_{k,l} \alpha_l
S_{j,l}$), for $0\leq i,j < Q$, and the $Q \times Q$ matrix
$U = S A\pi A S^{\,t}$.  The conclusion results from
$\pi = A^{-1}S^{-1}U {(S^{\,t})}^{-1}A^{-1}$ (resp.
$\pi =\rho^{-2} A^{-1}S^{-1}U {(S^{\,t})}^{-1}A^{-1}$).
\end{proof}

\begin{proof}[Proof of Theorem~\ref{thm.identifiabilityClass}]

  Let $P_{[n]}$ denote the probability distribution function of
  $(\Xn^o,R)$. We show that there exists a unique $(\alpha,\pi,\rho)$
  corresponding to $P_{[n]}$.

\paragraph{Identifiability of $\alpha$.}
Up to reordering, let $ t_1 < t_2 < \ldots < t_Q $ denote the
coordinates of the vector $t$ in the increasing order, we have :
$t_q=\mathbb{P}(\MA_{ij}=1, V_j=1|Z_{iq}=1)$.

Let $T$ denote the Vandermonde matrix defined by $T_{i,q}=t_q^i$, for
$0\leq i<Q$ and $1\leq q \leq Q$.  $T$ is invertible since the
coordinates of $t$ are all different.  For $i\geq1$,
$T_{i,q} =\mathbb{P}(\MA_{12}=1, \ldots, \MA_{1 i+1}=1, V_2=1, \ldots,
V_{i+1}=1| Z_{1q}=1)$. Let us also define
\begin{equation*}
v_i=\sum_{1\leq k\leq Q} \alpha_k t_k^i,\quad i=0,\ldots,2Q-1\enspace.
\end{equation*}
For $i \geq 1$,
$v_i=\mathbb{P}(\MA_{12}=1, \ldots, \MA_{1 i+1}=1, V_2=1, \ldots,
V_{i+1}=1)$.  Hence given $P_{[n]}$, $v_0=1$ and $v_1,\ldots,v_{2Q-1}$
are known. Furthermore, set $N$ the $(Q+1) \times Q$ matrix given by
$N_{i,j}=v_{i+j}$ for $0\leq i\leq j\leq Q$, and let $N_i$ denote the
square matrix obtained by removing the row $i$ from $N$. The
coefficients of $N_Q$ are
\begin{equation*}
N_{i,j}=v_{i+j}=\sum_{1\leq k \leq Q } t_k^i \alpha_k
t_k^j\enspace,\quad \mathrm{with}\quad 0 \leq  i,j < Q\enspace.
\end{equation*}
Defining the diagonal matrix $A=\mathrm{Diag}(\alpha)$, it comes
that $N_Q=TAT^{\,t}$, where $T$ and $A$ are invertible.
With $D_k=\det(N_k)$ and the polynomial $B(x)=\sum_{k=0}^Q
(-1)^{k+Q} D_k\, x^k$, it yields $D_Q=\det(N_Q)\neq0$ and the
degree of $B$ is equal to $Q$.

Set $C_i=(1,t_i,\ldots,t_i^Q)^t$ and let us notice that $B(t_i)$ is
the determinant of the square matrix produced when appending $C_i$ as
last column to $N$.  The $Q+1$ columns of this matrix are linearly
dependent, since they are all linear combinations of the $Q$ vectors
$C_1$, $C_2$, $\ldots$, $C_Q$.  Hence $B(t_i)=0$ and $t_i$ is a root
of $B$ for every $1\leq i\leq Q$.  This proves that
$B=D_Q\prod_{i=1}^Q(x-t_i)$.  Then, one knows that
$t=(t_1,\ldots,t_Q)$ (as the roots of $B$ defined from $N$) and $T$.
It results that $A= T^{-1} N_Q (T^{\,t})^{-1}$, which yields a unique
$(\alpha_1,\ldots,\alpha_Q)$.

\paragraph{Identifiability of $\rho$.} 
Up to reordering, let $ o_1 < o_2 < \ldots < o_Q $ denote the
coordinates of the vector $o$ in the increasing order, then
$s_q=\mathbb{P}(\MA_{ij}=1, V_i=1|Z_{iq}=1)=\rho_q o_q$.  Let $O$
denote the Vandermonde matrix defined by $O_{i,q}=o_q^i$, for
$0\leq i<Q$ and $1\leq q \leq Q$.  $O$ is invertible since the
coordinates of $o$ are all different.  For $i\geq1$,
$O_{i,q} =\mathbb{P}(\MA_{12}=1, \ldots, \MA_{1 i+1}=1| Z_{1q}=1)$.
Let us also define
\begin{equation*}
u_i=\sum_{1\leq k\leq Q} \rho_k \alpha_k o_k^i,\quad i=0,\ldots,2Q-1\enspace.
\end{equation*}
For $i \geq 1$,
$u_i=\mathbb{P}(\MA_{12}=1, \ldots, \MA_{1 i+1}=1, V_1=1)$.  Hence
given $P_{[n]}$, $u_0=1$ and $u_1,\ldots,u_{2Q-1}$ are
known. Furthermore, set $M$ the $(Q+1) \times Q$ matrix given by
$M_{i,j}=u_{i+j}$ for every $0\leq i\leq Q$ and $0\leq j<Q$, and let
$M_i$ denote the square matrix obtained by removing the row $i$ from
$M$.
The coefficients of $M_Q$ are
\begin{equation*}
M_{i,j}=u_{i+j}=\sum_{1\leq k \leq Q } o_k^i \alpha_k \rho_k
o_k^j\enspace,\quad \mathrm{with}\quad 0 \leq  i,j < Q\enspace.
\end{equation*}
Defining the diagonal matrix $B=\mathrm{Diag}(\rho)$, it comes that
$M_Q=OABO^{\,t}$, where $O$, $B$ and $A$ are invertible. Using the
same algebraic argument than for the identifiability of $\alpha$, it
results that $B= A^{-1}O^{-1} M_Q (O^{\,t})^{-1}$, which yields,
because of the identifiability of $\alpha$, a unique
$(\rho_1,\ldots,\rho_Q)$.

\paragraph{Identifiability of $\pi$.}

For $0 \leq i,j <Q $, let us introduce $U_{i,j}$ the probability that
the first row of $\MA^o$ begins with $i+1$ occurrences of 1, and the
second row of $\MA^o$ ends up with $j$ occurrences of 1.
\begin{multline*}
U_{i,j}=\mathbb{P}\Big(\left\{ \MA_{12}=1, \ldots, \MA_{1 i+2}=1, V_2=1, \ldots, V_{i+2}=1 \right\}\bigcap \\ \left\{ \MA_{2 n-j}=1, \ldots, \MA_{2 n}=1, V_{n-j}=1, \ldots, V_{n}=1 \right\} \Big),
\end{multline*}
Then,
$U_{i,j}=\sum_{k,l} T_{i,k} \alpha_k \pi_{k,l} \rho_k \alpha_l
T_{j,l}$, for $0\leq i,j < Q$, and the $Q \times Q$ matrix
$U = TA\pi A B T^{\,t}$.
The conclusion results from
$\pi = A^{-1}T^{-1}U {(T^{\,t})}^{-1}B^{-1}A^{-1}$.

\end{proof}

%%% Local Variables:
%%% TeX-master: "TBC_JASA_17.tex"
%%% End:
