# Supplementary material for: Variational Inference for Stochastic Block Models from Sampled Data
Source: arXiv:1707.04141 source file (2019-01-09)
Supplement: Supplementary file 2 [file appendix_more_ER.tex]

\subsection{Additional results for the ER Protein-Protein Interaction
  network}
\label{sec:moreER}

In this appendix, we provide more details on the NMAR clustering of
the ER network discussed in Section \ref{sec:er1}.  We represent the
estimated connectivity matrix $\hat{\pi}$ in
Figure~\ref{fig:graph_esr1_nmar} for NMAR, which exhibits a
network-structure with 13 blocks (or sets of proteins) the sizes of
which can be sketched from Figure~\ref{fig:alluvial_esr1}.  In
Figure~\ref{fig:graph_all_esr1_nmar}, we represent on the same matrix
the network with the original missing data and the imputed missing
dyads with the variational parameters $\nu$. Interestingly, many of
the imputed values are close to $1$, which might help validating some
relationships which were still uncertain in the biological
literature. Figure~\ref{fig:alluvial_esr1} shows that the MAR
clustering leads to a large cluster (block 3) which is mainly split
into 4 blocks in the NMAR clustering (blocks 3, 4, 6 and 13).

\begin{figure}[htbp!]
  \centering
  \begin{subfigure}[b]{.45\textwidth}
    \centering
      \begin{tabular}{ccc}
     \rotatebox{90}{\hspace{1.7cm} \small MAR estimated clusters} & \includegraphics[width=.8\textwidth]{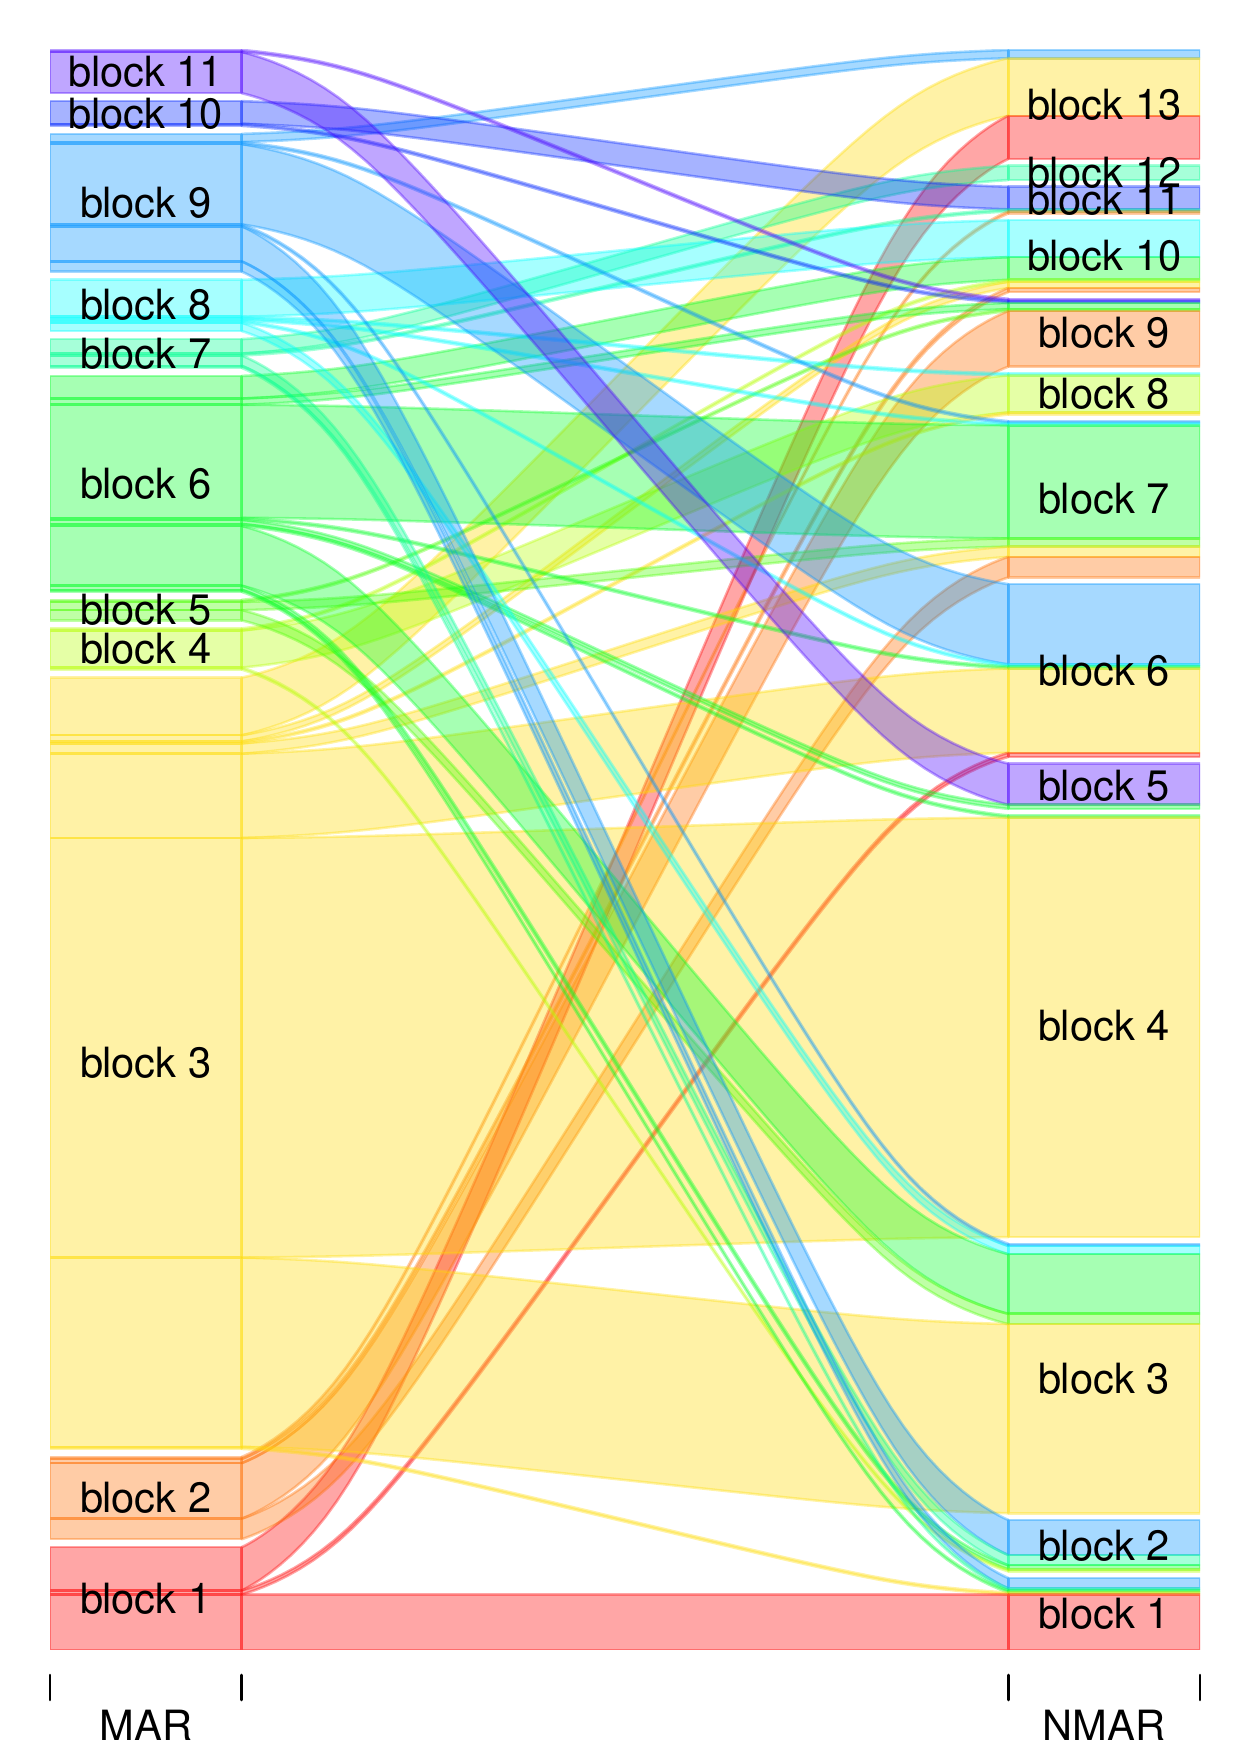}
    &  \rotatebox{90}{\hspace{1.7cm} \small NMAR estimated clusters}
  \end{tabular}
    \caption{Clustering  comparison   between  MAR  and  NMAR (11 vs 13 blocks).}
    \label{fig:alluvial_esr1}
  \end{subfigure}\hfill
  \begin{subfigure}[b]{.5\textwidth}
    \centering
    \includegraphics[width=.85\textwidth]{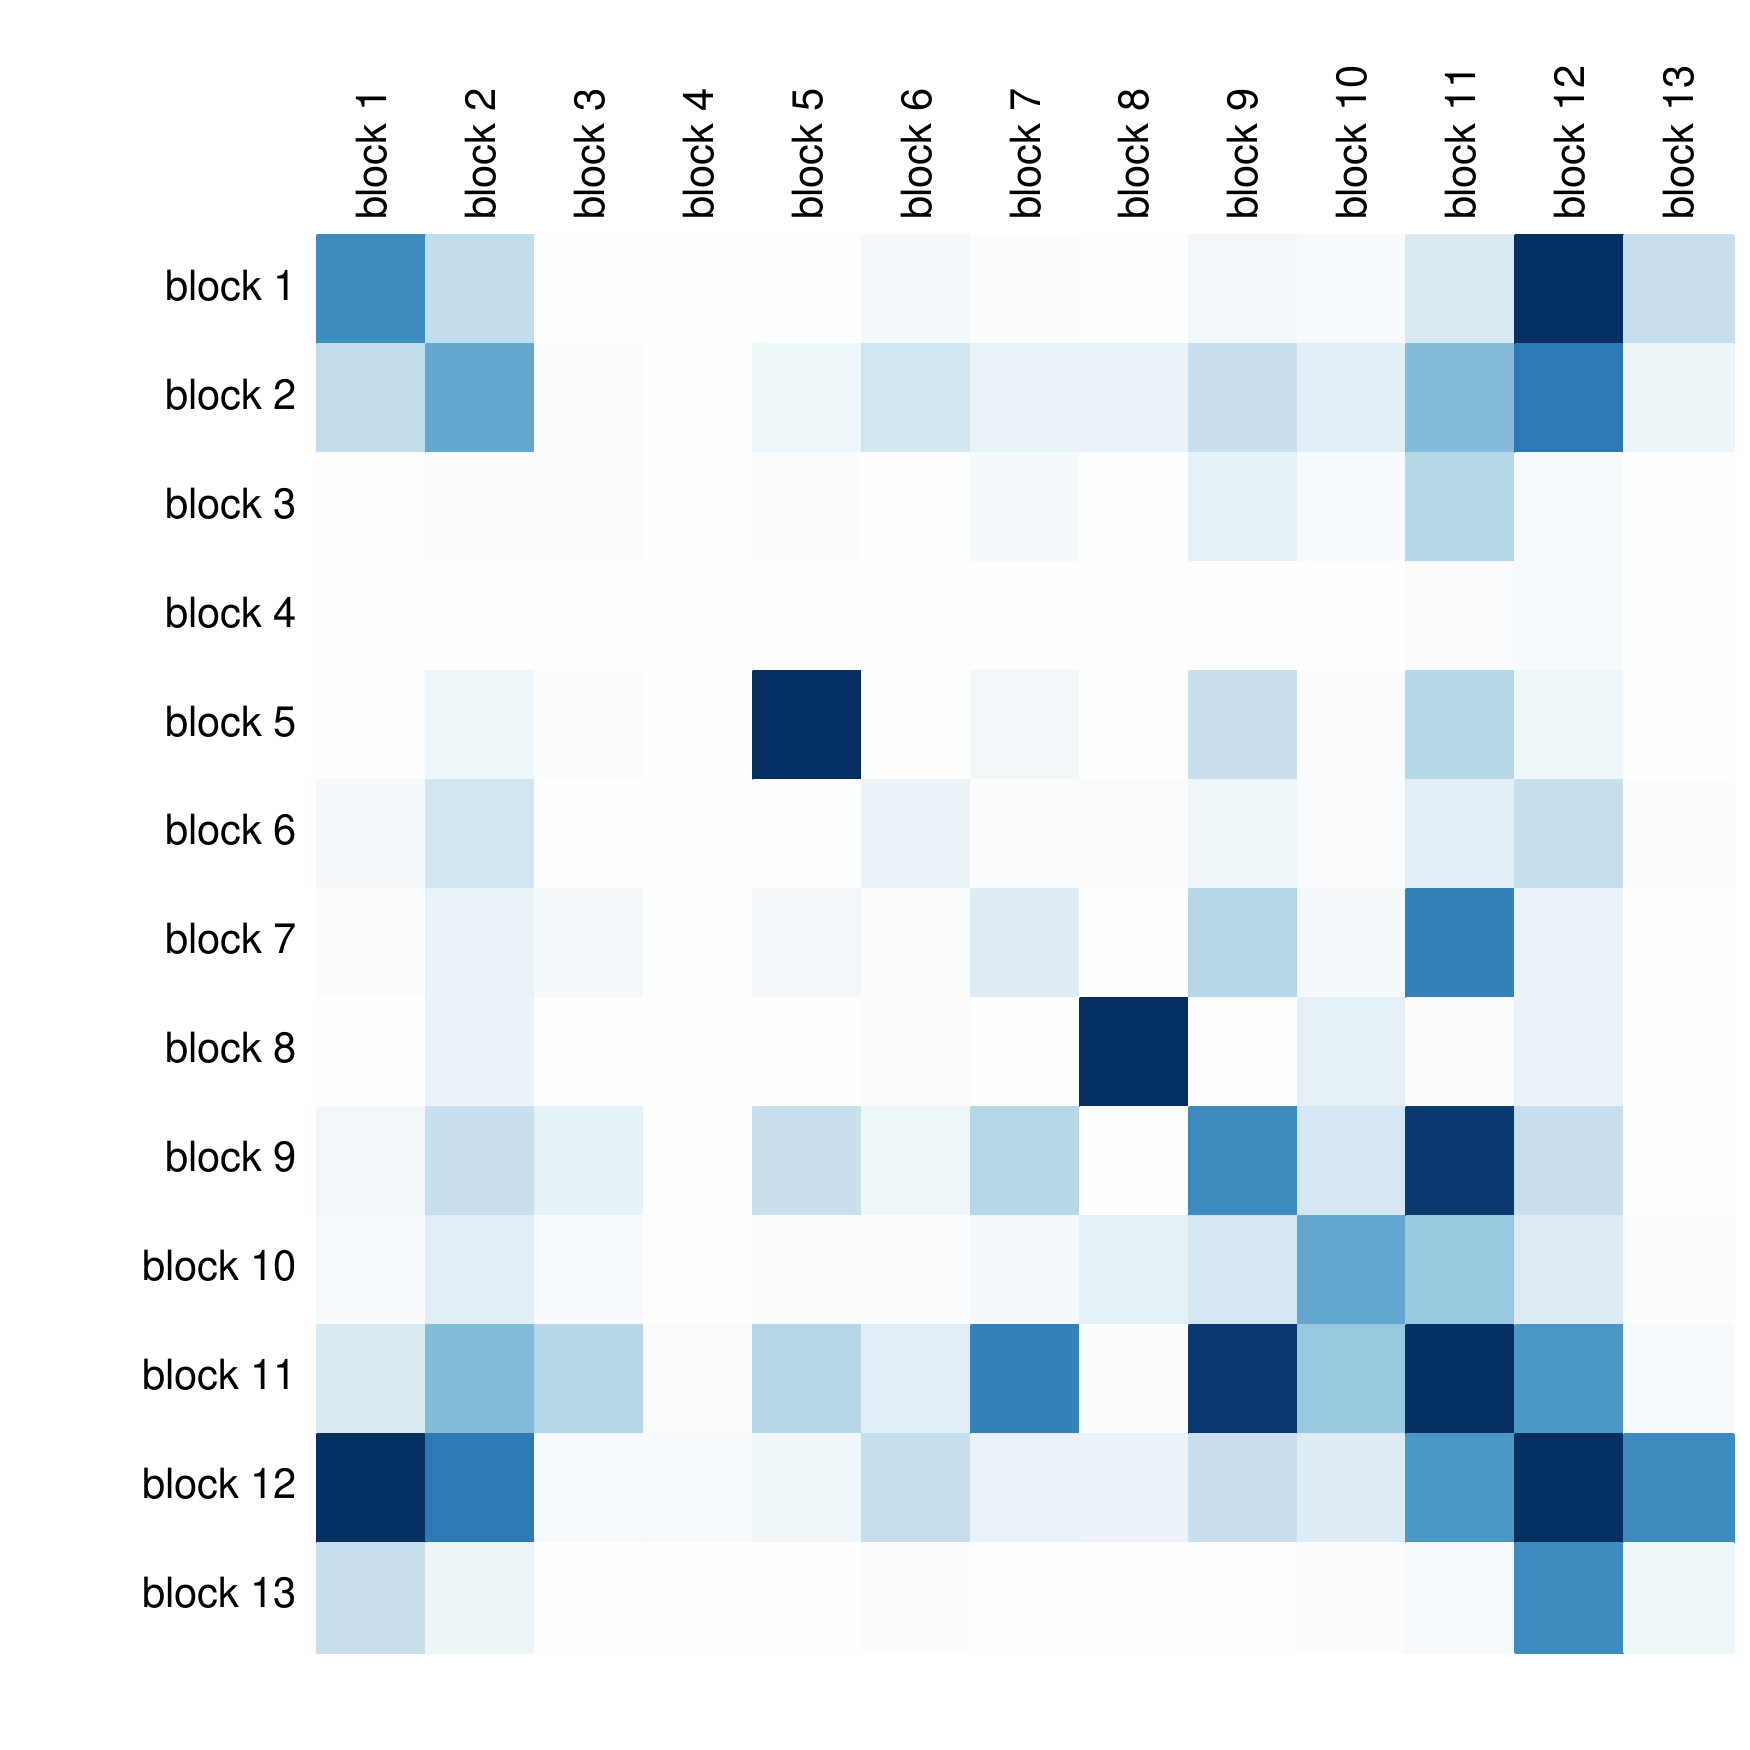}
    \caption{Matrix  of connectivity  $\hat{\pi}$  for NMAR  inference
      (double standard) ; intensity of the color is proportional to the probability of
      connection   between  blocks.}
    \label{fig:graph_esr1_nmar}
  \end{subfigure}
  \begin{subfigure}[c]{\textwidth}
    \centering
      \includegraphics[width=\textwidth]{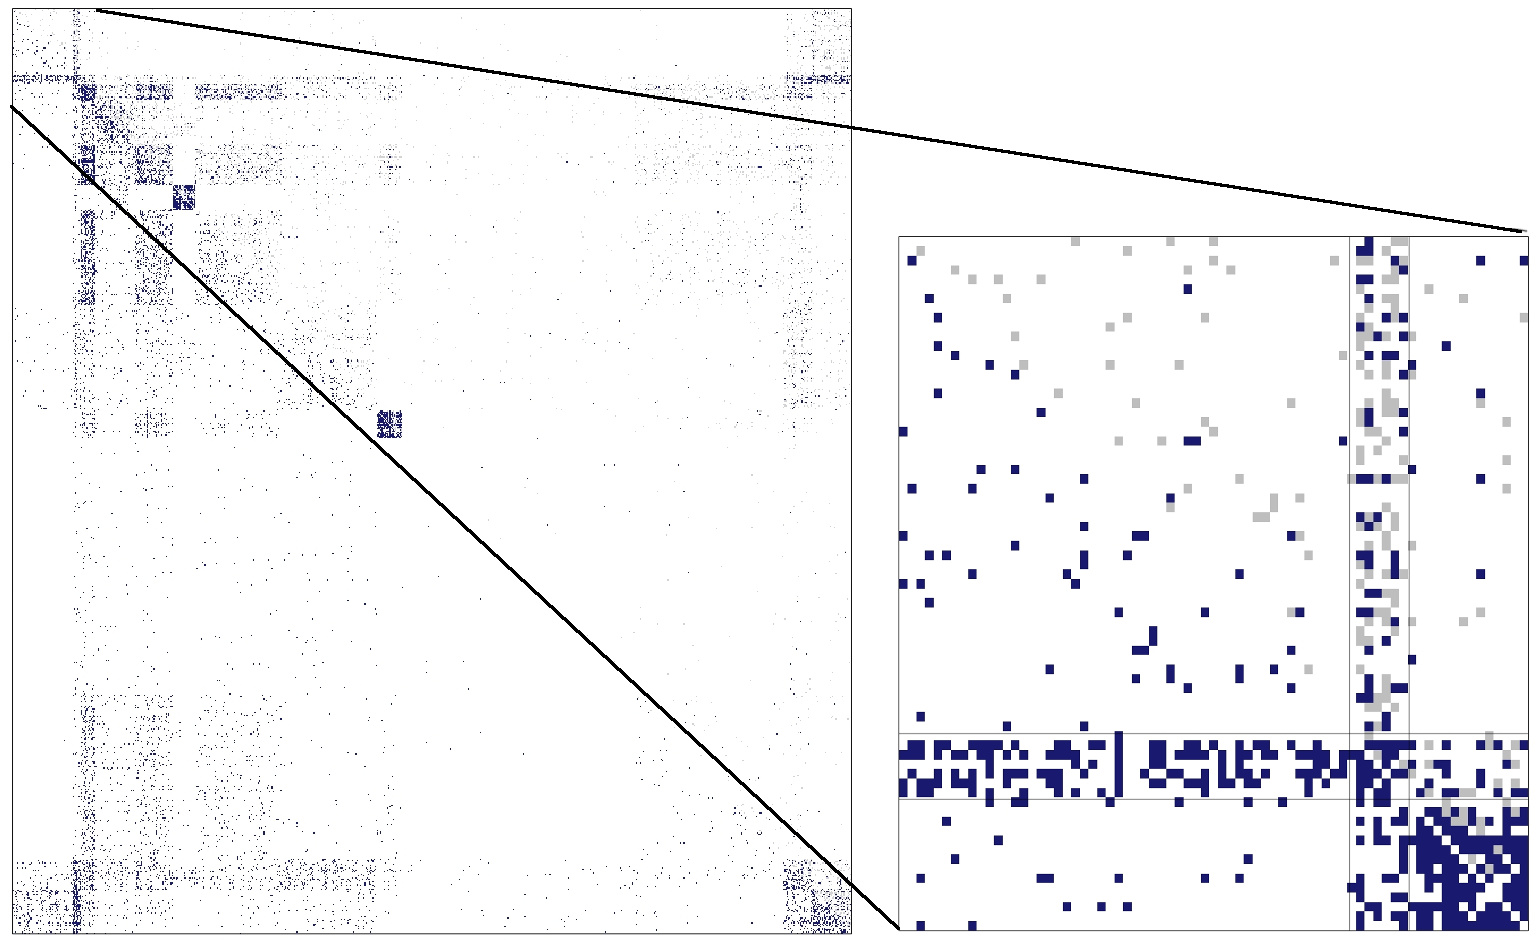}
      \caption{ER  PPI network  reordered  by  blocks inferred  with
        SBM with NMAR modeling. Left panel: original data with
        \texttt{NA} entries colored in gray (upper triangle) and data imputed with
        $\nu_{ij}$ (lower triangle); right panel: zoom of blocks (1,2,3).}
    \label{fig:graph_all_esr1_nmar}
  \end{subfigure}

  \caption{ER PPI network analysis with SBM under missing data conditions}
\end{figure}
