# Supplementary material for: Variational Inference for Stochastic Block Models from Sampled Data
Source: arXiv:1707.04141 source file (2019-01-09)
Supplement: Supplementary file 3 [file appendix_simu_nmar.tex]

\subsection{Simulations for star degree ans star samplings}
\label{appendix:simu-nmar}

With node-centered samplings such as star-degree and class samplings,
it is more difficult to find configurations different from MAR
sampling designs: with dyad-centred double-standard design, the
sampling parameters were directly related to the probability of an
edge conditionally on the observation of the corresponding dyad, which
is no longer the case for the node-centered designs. The sampling
designs being hardly different from a MAR design, the NMAR inference
does not show much improvement compared to the MAR inference. Still,
we exhibit some interesting situations where star degree and class
samplings deserve an appropriate treatment, presented herein.  We
simulate networks with $n=100$ nodes under an affiliation topology
with intra-community probability (resp. inter community probability)
equal to $0.5$ (resp. $0.05$) and $\alpha = (0.25, 0.5,
0.25)$. Sampling parameters are chosen such that
$\psi=(a,b) = (-3.6, 0.1)$ for star degree sampling, which makes nodes
with highest degrees preferably selected.  In class sampling, these
parameters are set to
$\psi=(\rho_1, \rho_2, \rho_3) = (0.75, 0.5, 0.05)$, which makes nodes
from the largest block and from a small block preferably selected
while the other small block is under-sampled.  In Figure
\ref{fig:simu_other_nmar}, the estimation errors and the ARI are
pictured for both cases.  The sampling rates (i.e.  rates of observed
dyads over total number of dyads) lie in the intervals $[0.558,0.844]$
for class sampling and $[0.162,0.622]$ for star degree sampling. These
two intervals arise from the values of the parameter $\psi$ explored
for these two designs.  We compare the performances of Algorithm
\ref{algo:vem:nmar} to an oracle (when inference is conducted via a
classical VEM algorithm on a fully observed network) and with
Algorithm \ref{algo:vem:mar}.  When facing NMAR condition, Algorithm
\ref{algo:vem:nmar} shows a slight improvement over Algorithm
\ref{algo:vem:mar} even if it remains far from the oracle.
% , which is designed  for handling missing data under
% MAR conditions, altough we are here  in NMAR conditions. 
% It allows us
% to show the  importance of taking into account the  sampling design in
% the inference  process when  facing NMAR  conditions.  Again,  we show
% that  Algorithm \ref{algo:vem:nmar}  manages  to produce  satisfactory
% estimates.

\begin{figure}[htbp!]
	\centering
   \begin{tabular}{c@{\hspace{.03mm}}c@{\hspace{.03mm}}c@{\hspace{.03mm}}c@{\hspace{.03mm}}c@{\hspace{.03mm}}c@{\hspace{.03mm}}c}
     & {\small $\|\hat{ \pi} - \pi \|_F / \| \pi\|_F$} & \hspace{0.5cm} & \small \textbf{ARI}$(Z, \hat{Z})$ & \\
     \rotatebox{90}{\hspace{1.5cm} \small class} & \includegraphics[width=.35\textwidth]{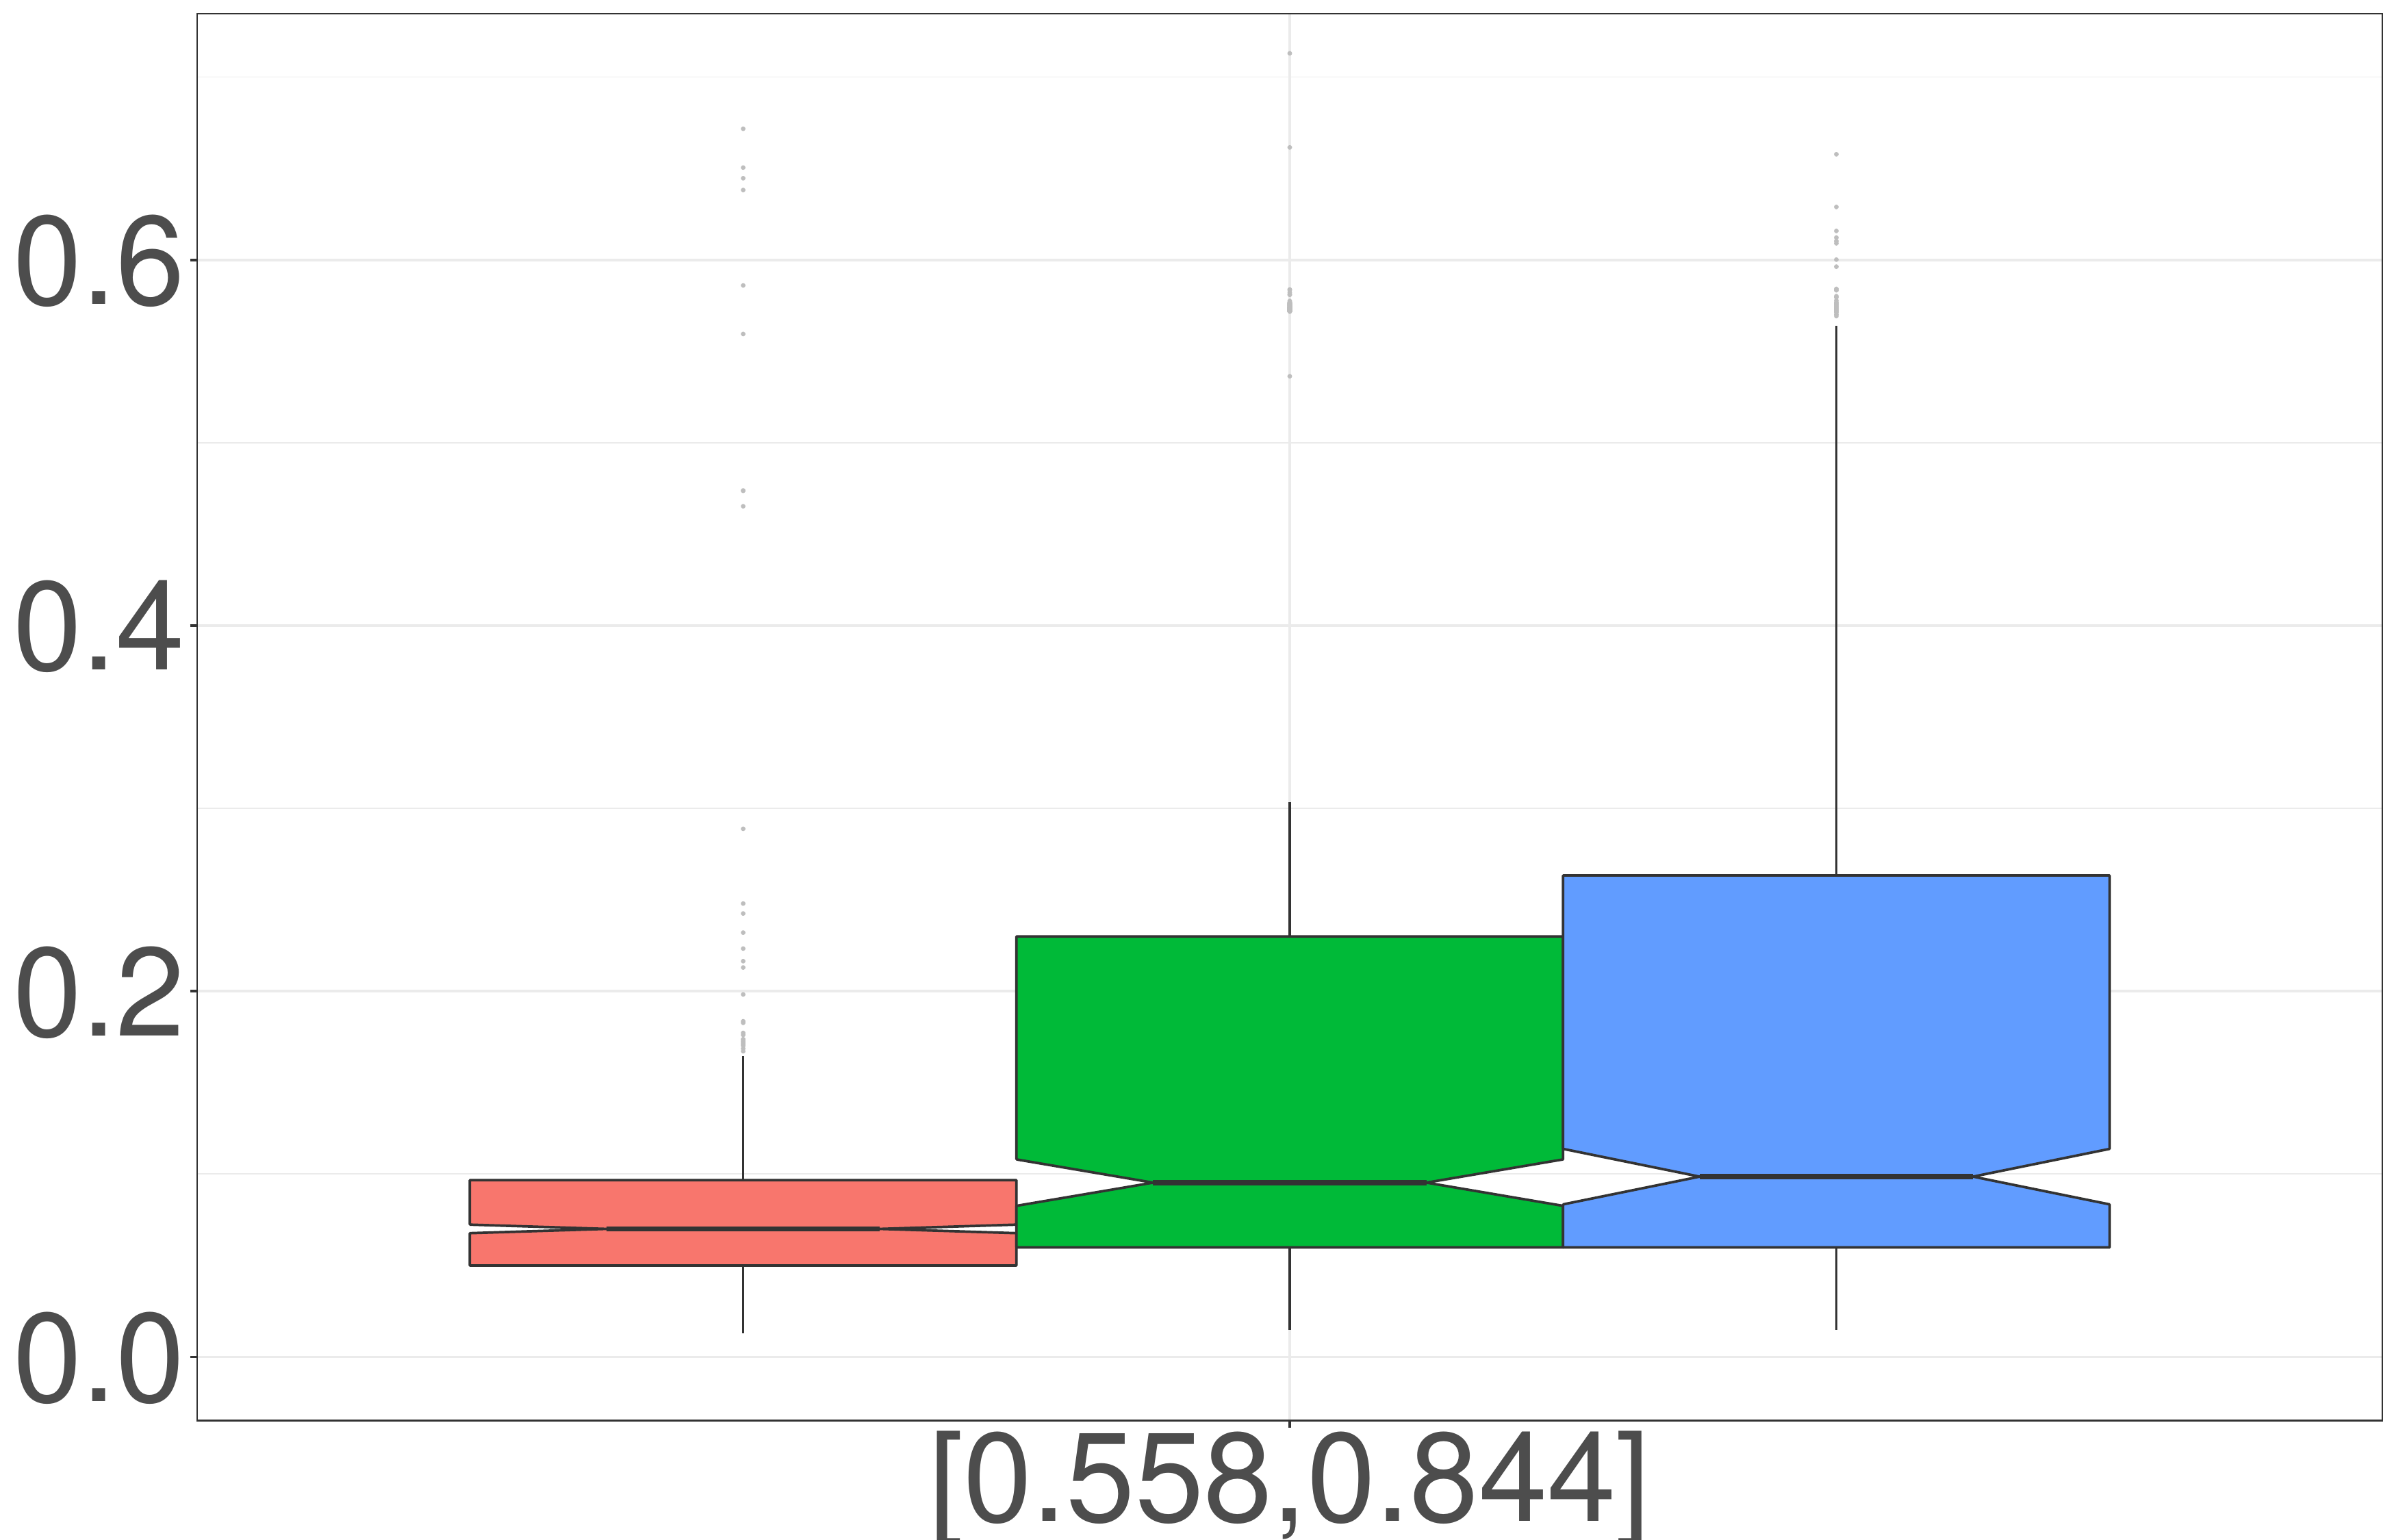} & \rotatebox{90}{} &
 	 \includegraphics[width=.35\textwidth]{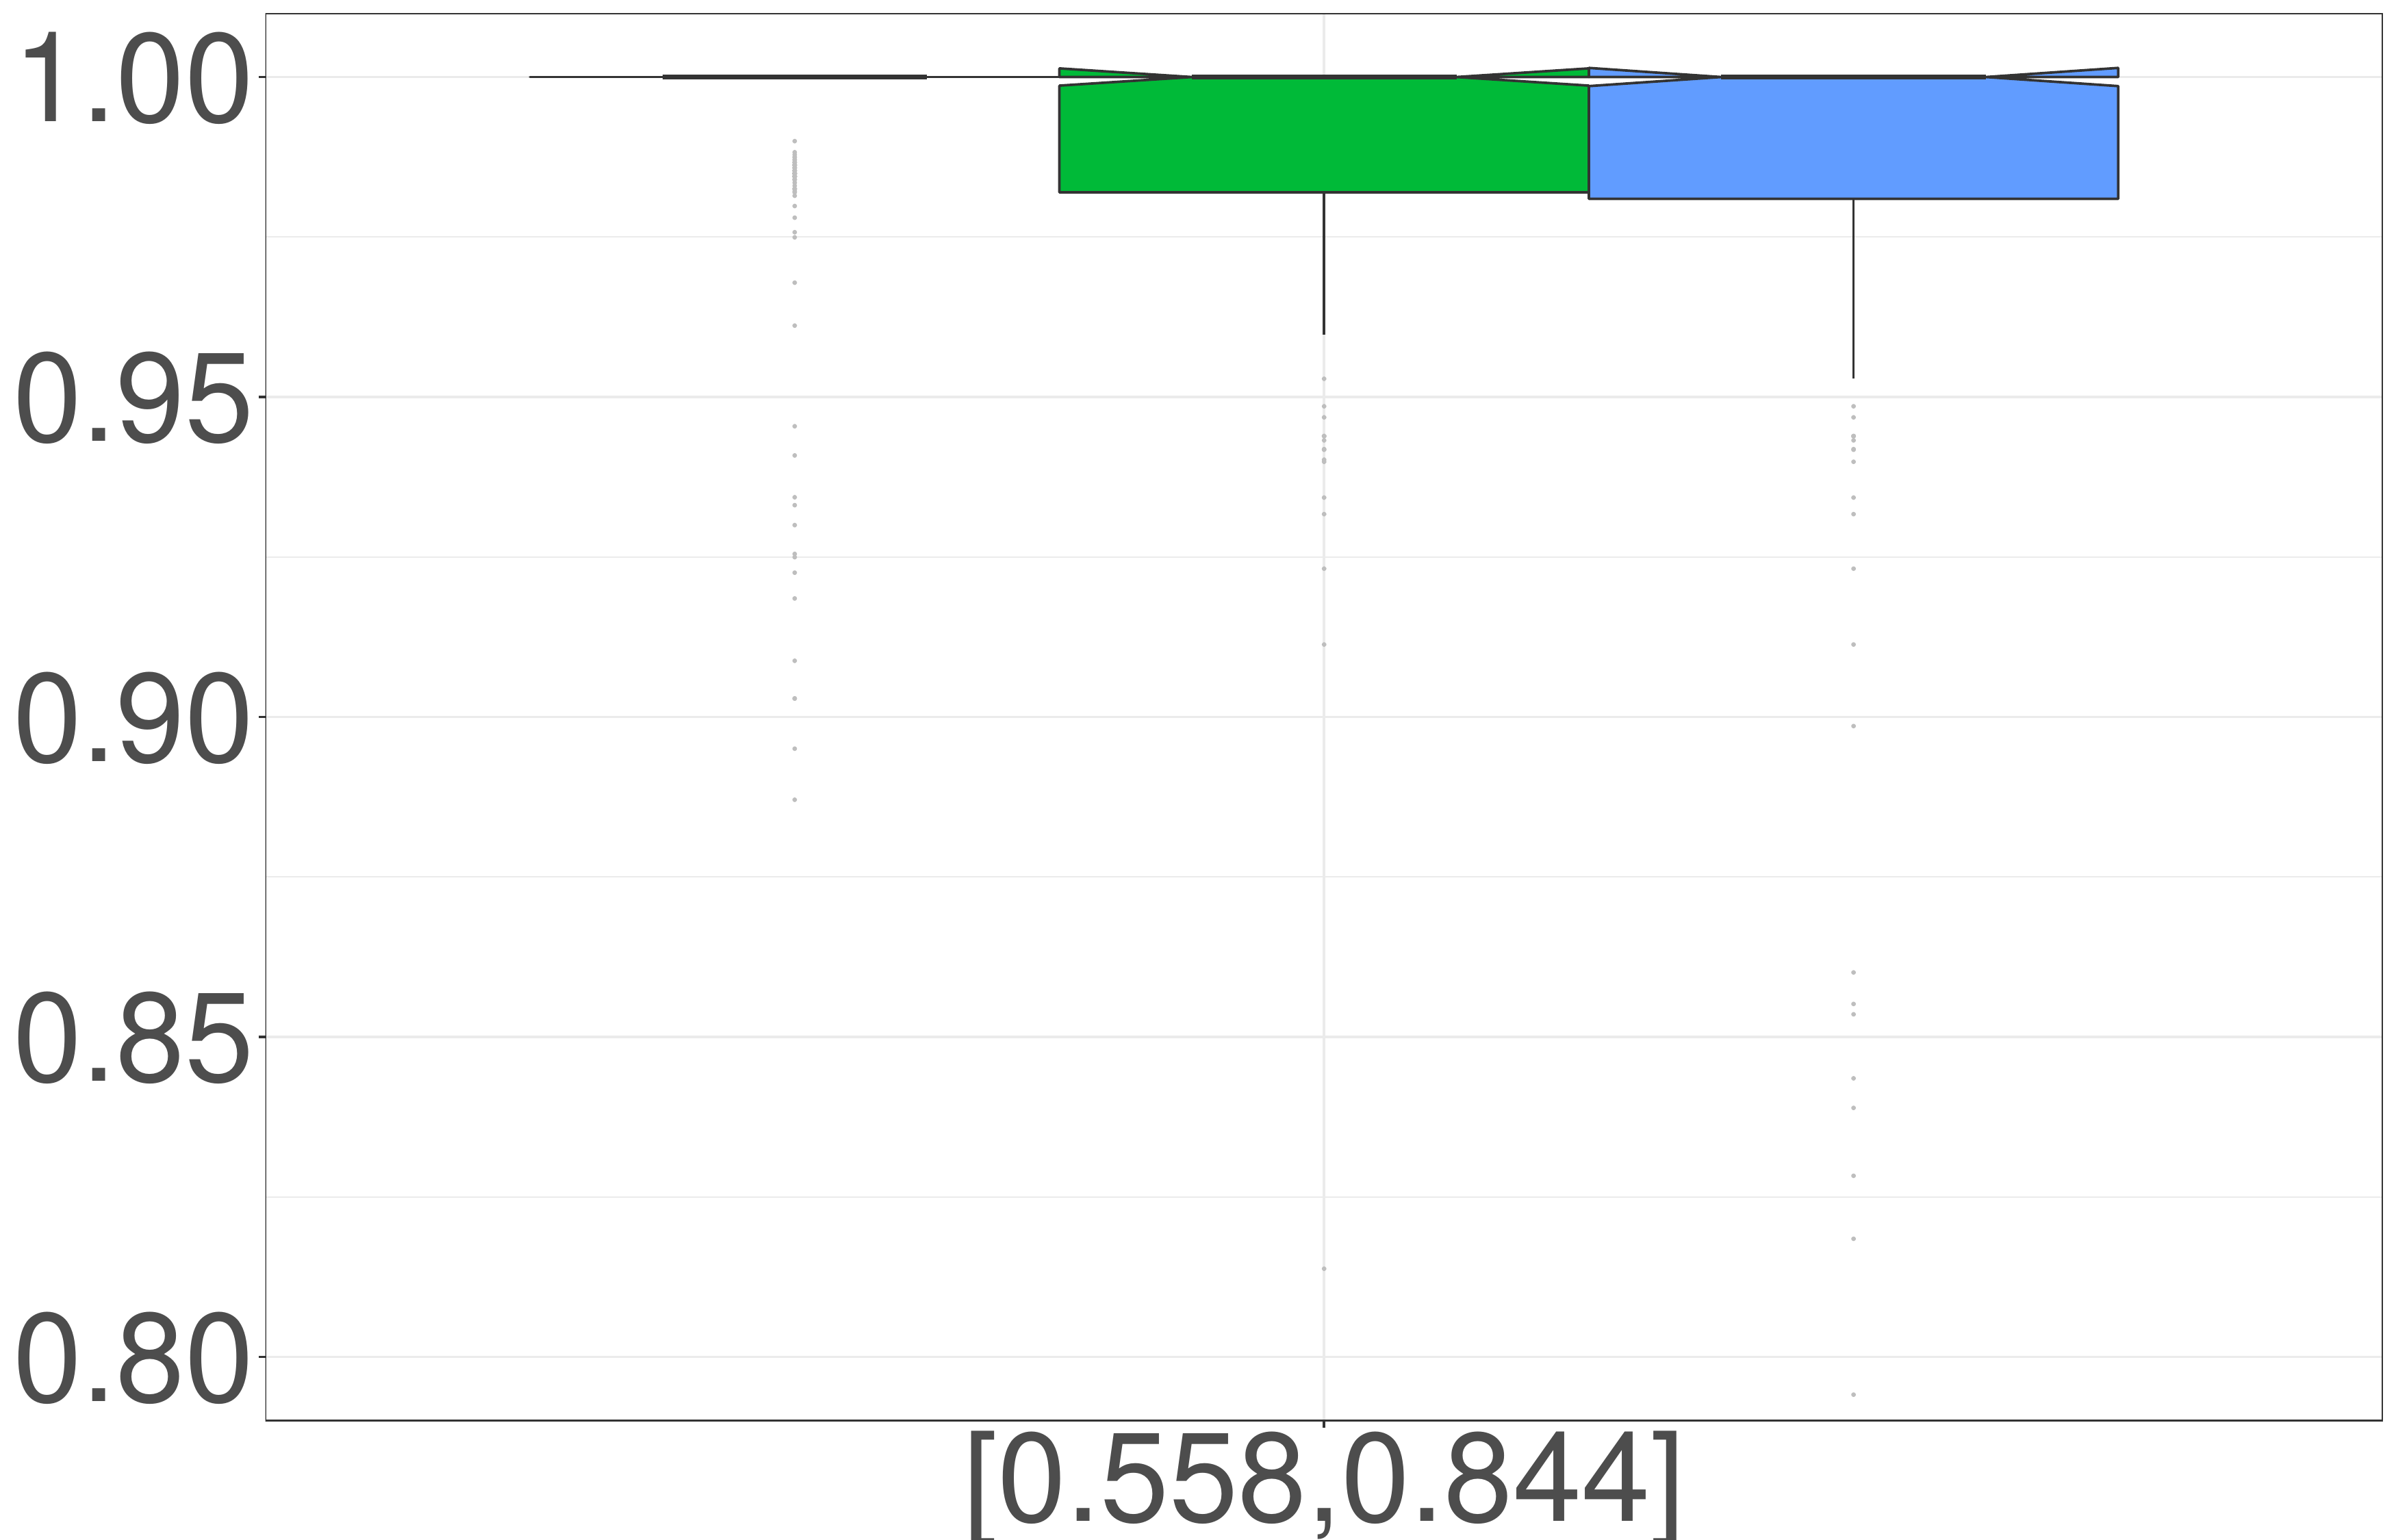} & \multirow{2}{*}{\quad \includegraphics[width=.08\textwidth]{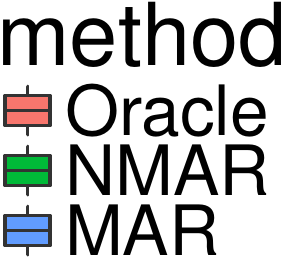}} \\ 
	\rotatebox{90}{\hspace{1.5cm} \small star degree} & \includegraphics[width=.35\textwidth]{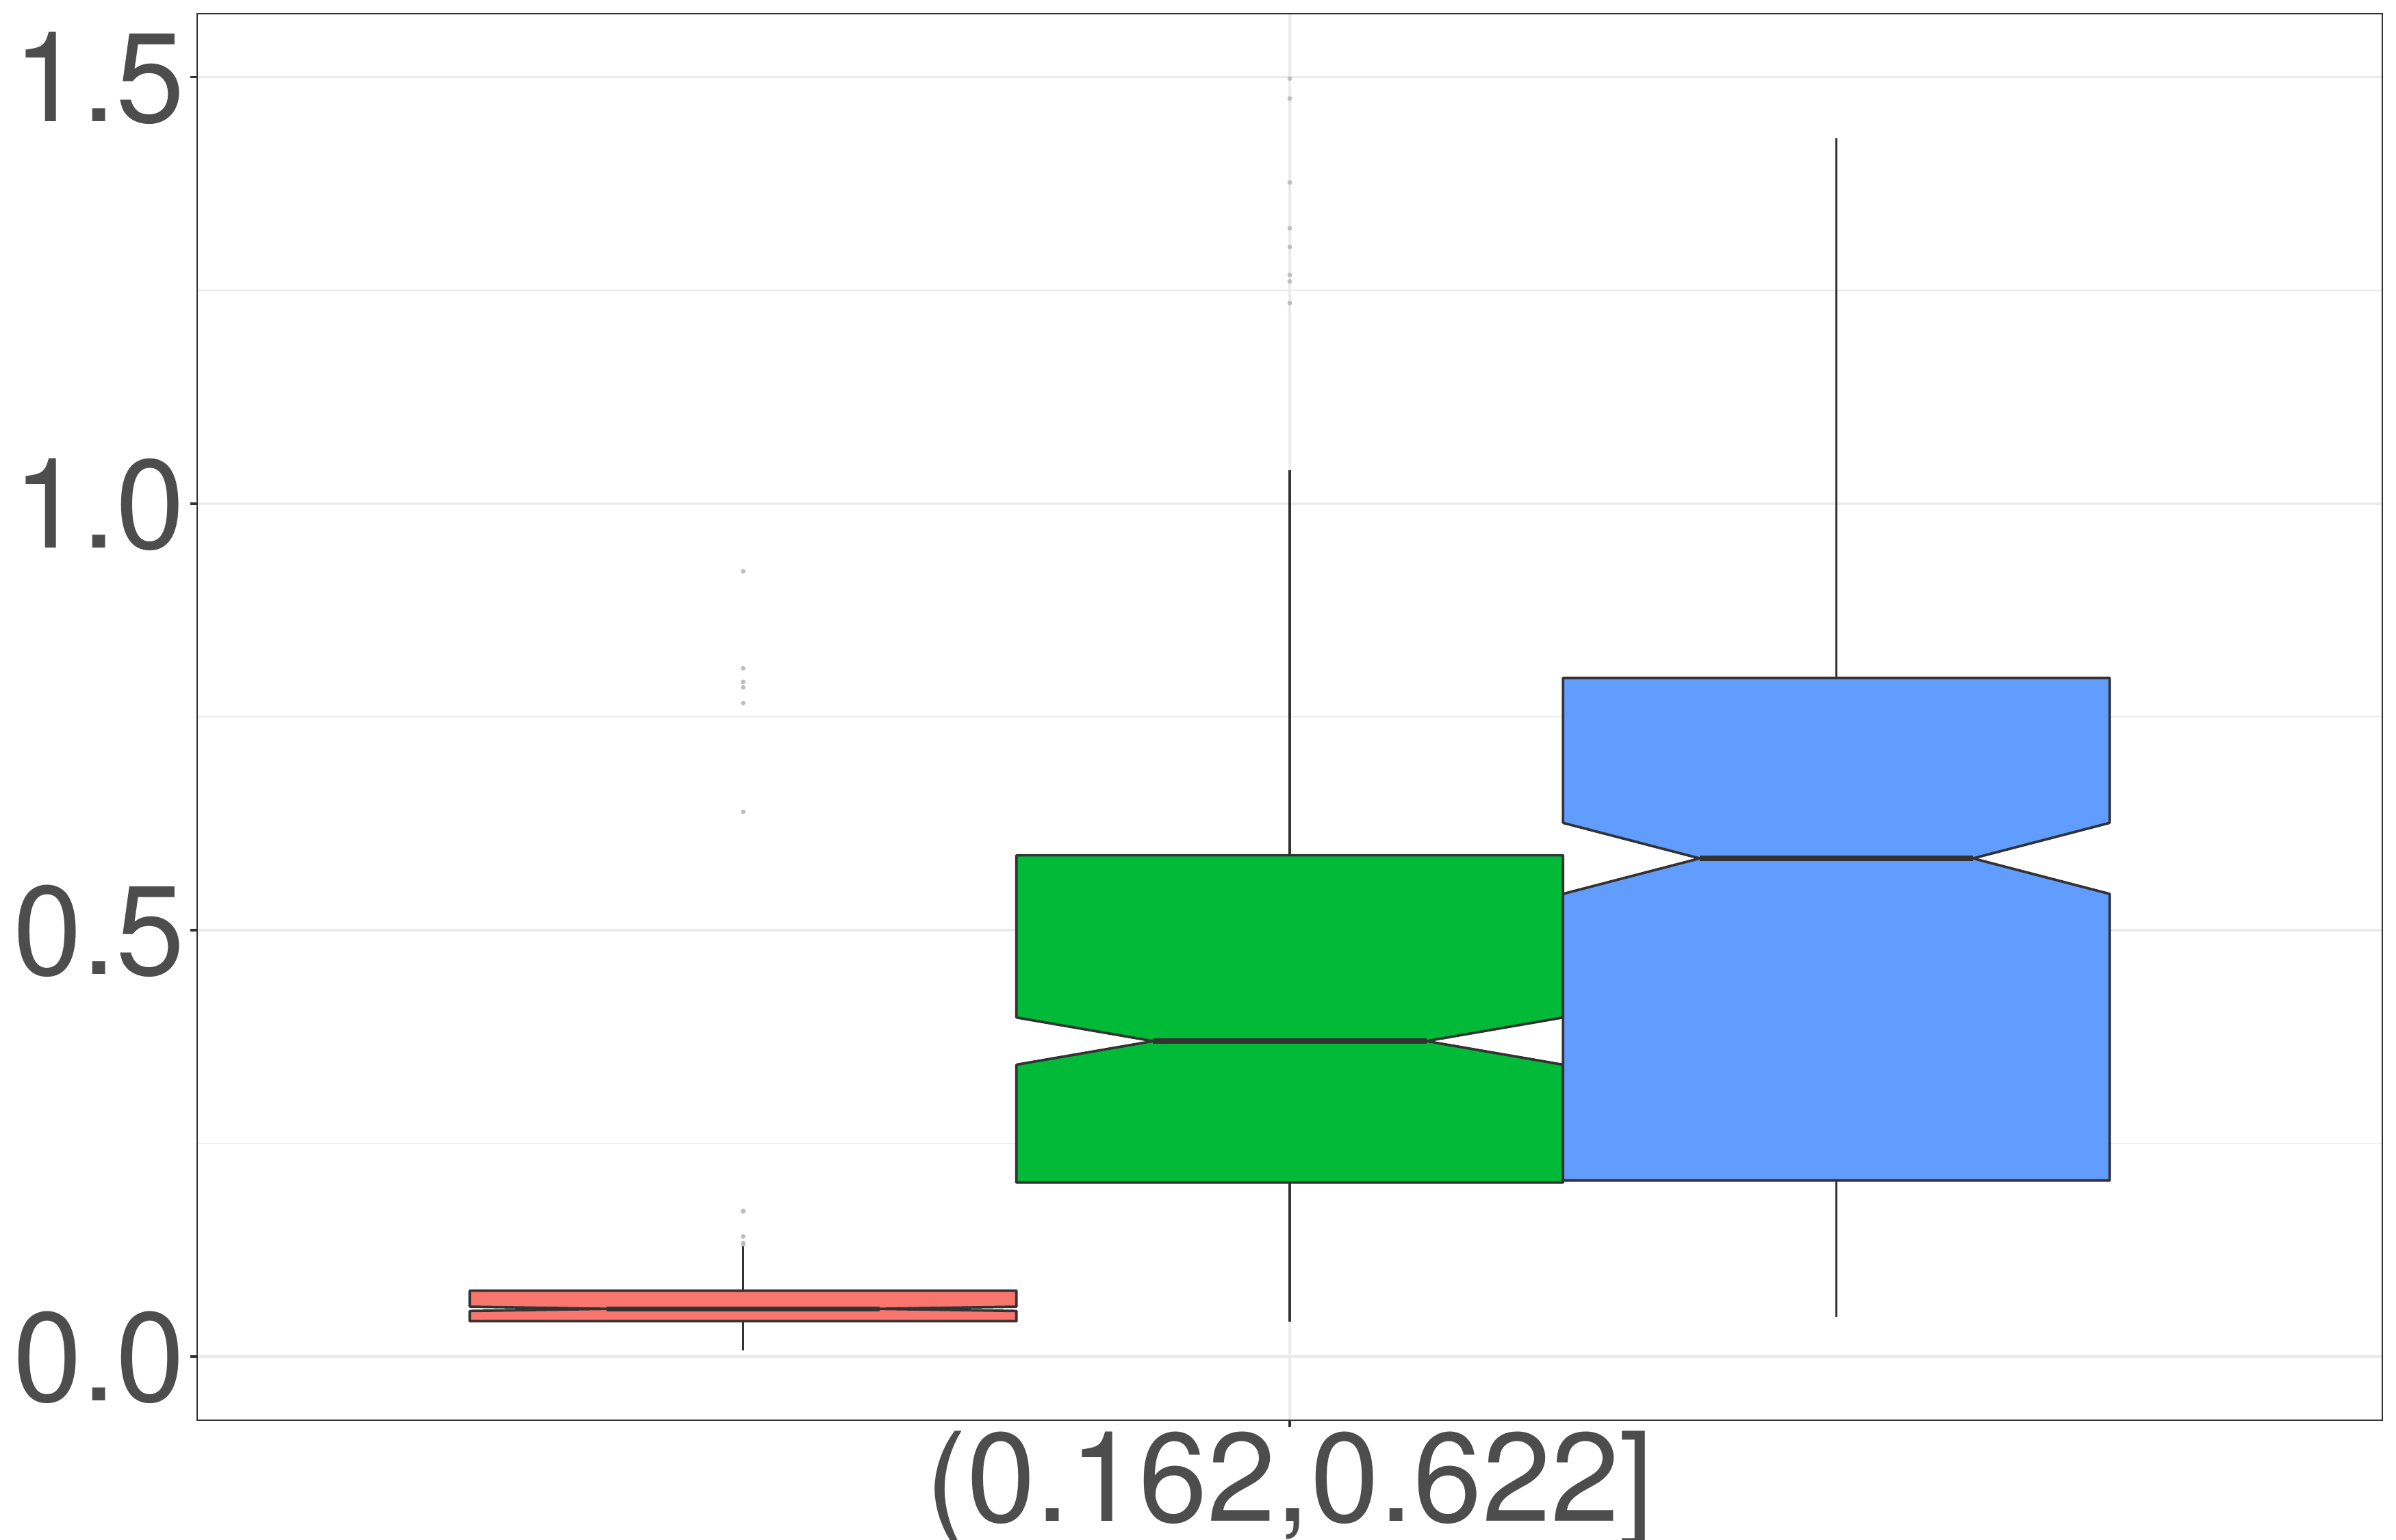} & \hspace{0.5cm} &
	 \includegraphics[width=.35\textwidth]{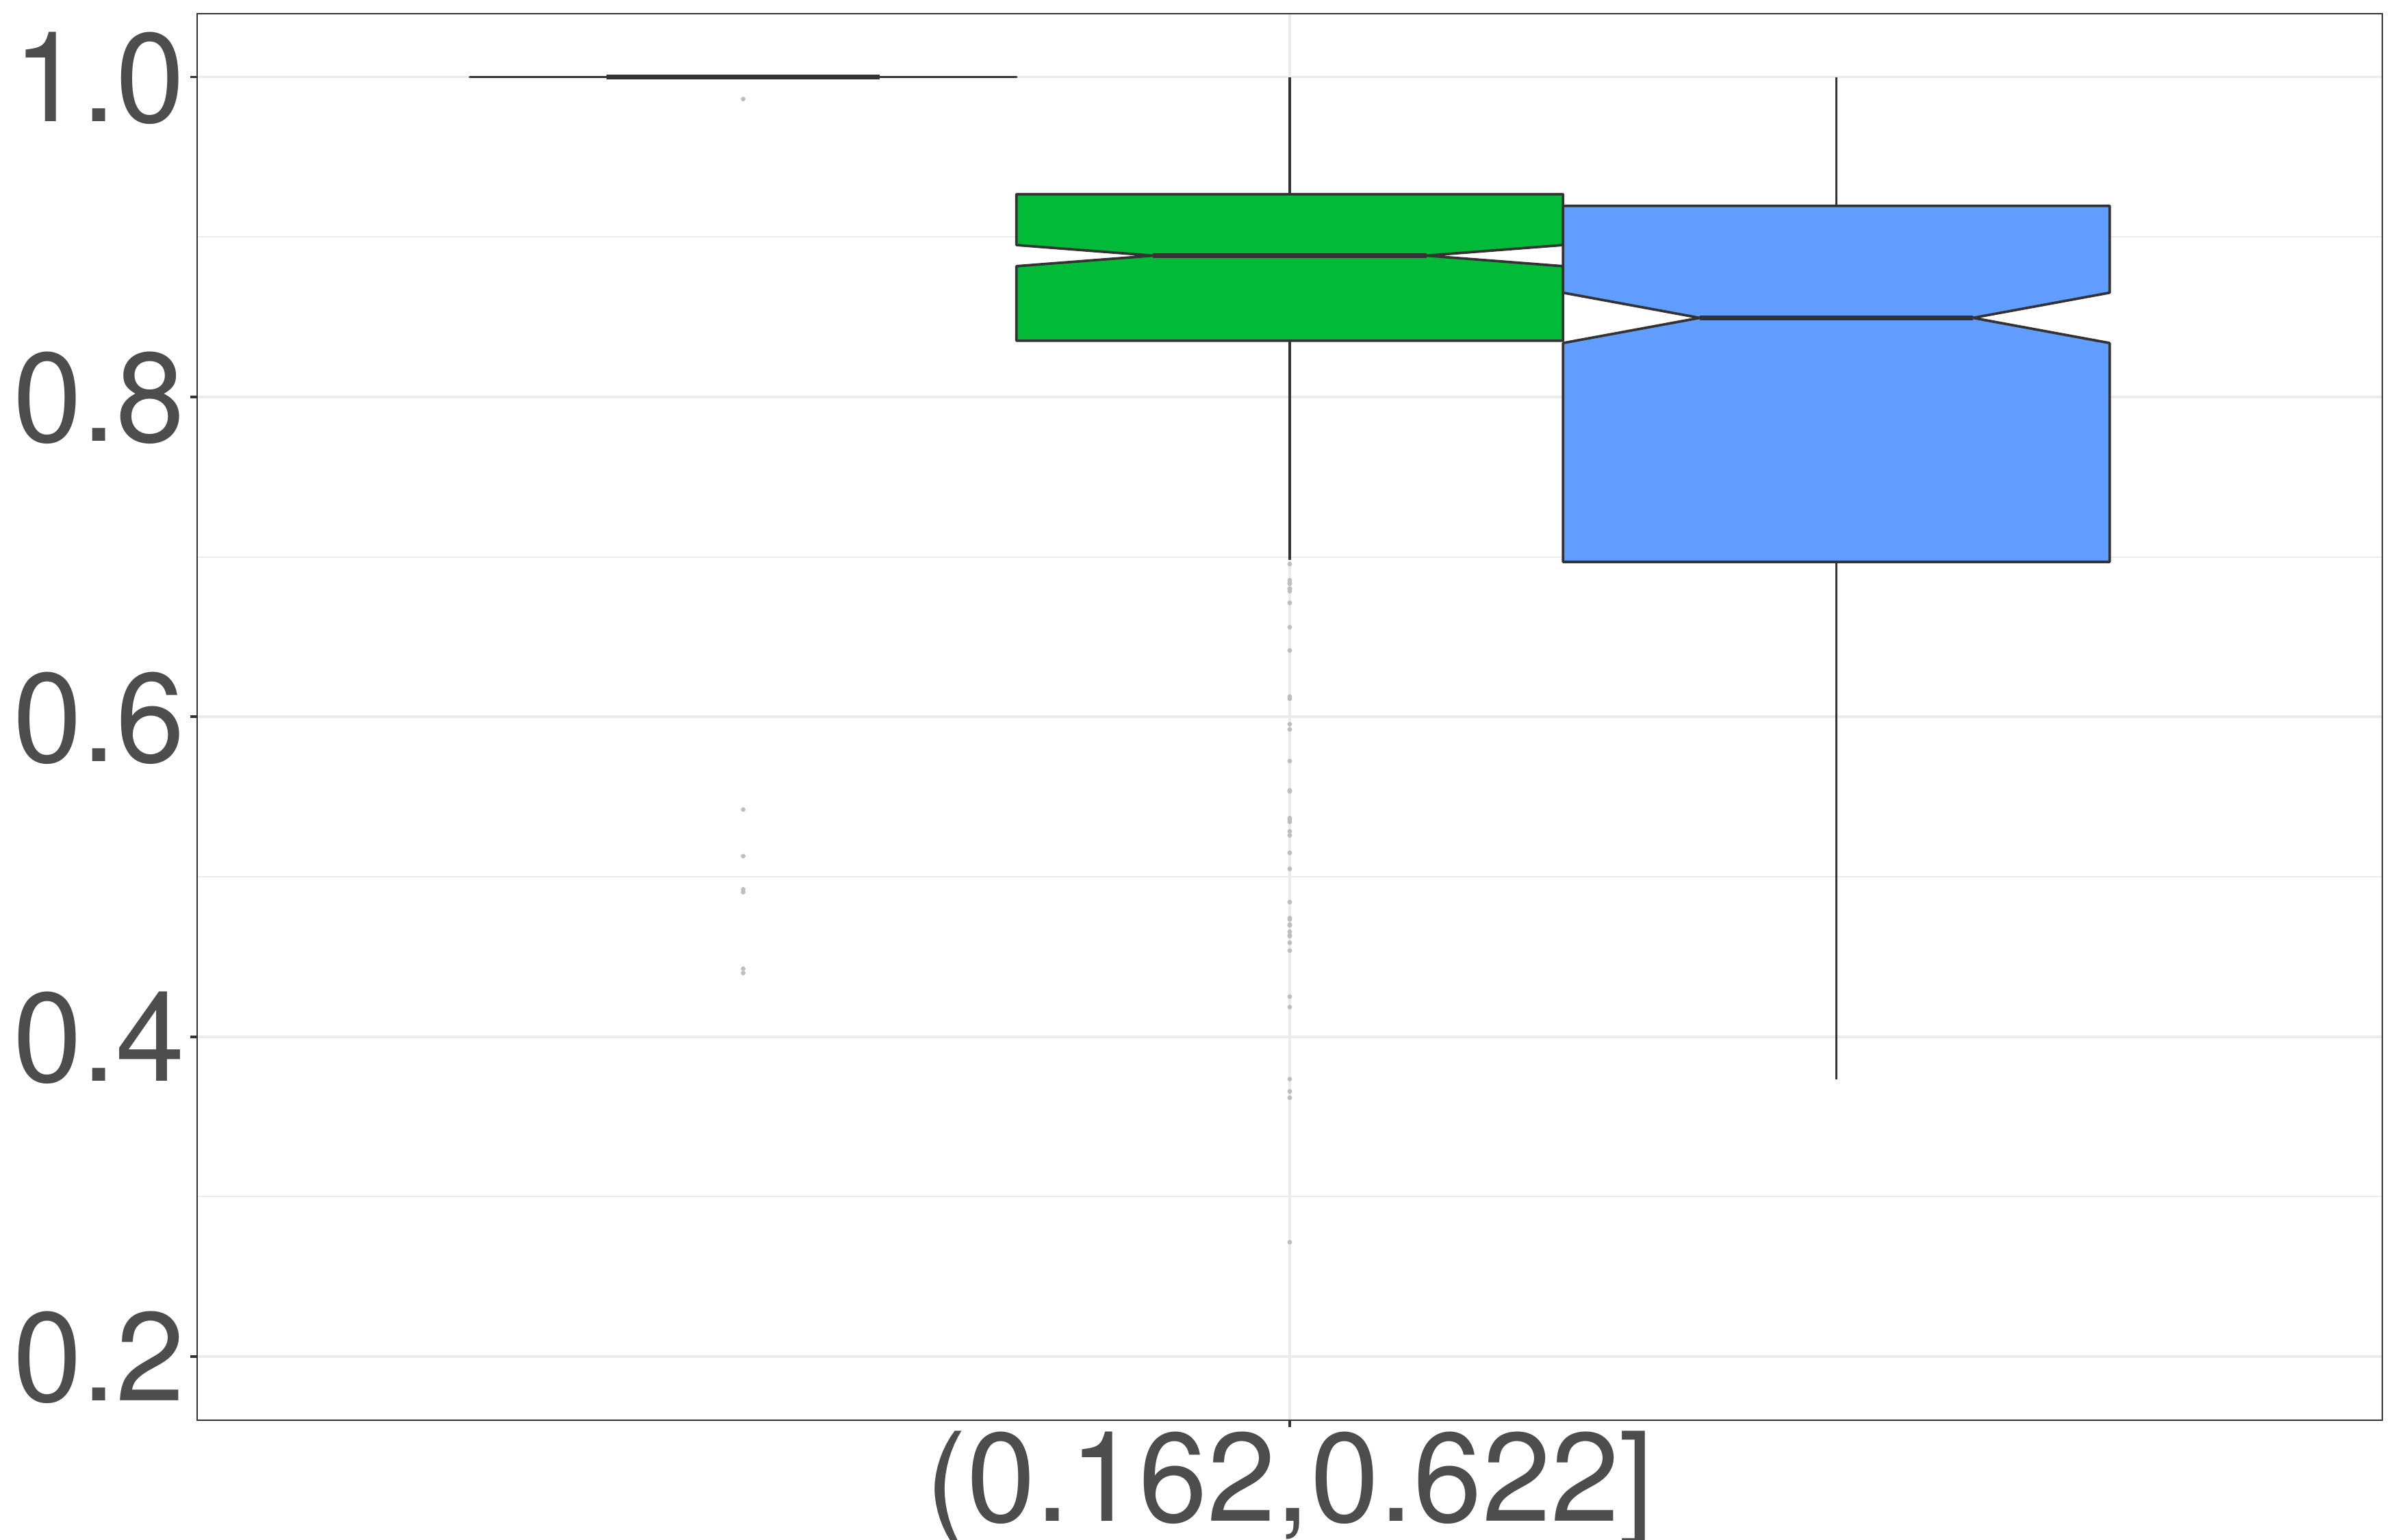} &  \\
	& \multicolumn{3}{c}{Proportion intervals of observed dyads} & \\
	\end{tabular}    
   \caption{Estimation error  of  $\pi$  and ARI averaged over 500
    simulations in star degree and class settings. The topology is affiliation with $\epsilon = 0.05$.}
	\label{fig:simu_other_nmar}
\end{figure}
