# Supplementary material for: Variational Inference for Stochastic Block Models from Sampled Data
Source: arXiv:1707.04141 ancillary file (2019-01-09)
Supplement: Supplementary file 4 [file Supplementary.pdf]

# Variational Inference for Stochastic Block Models from Sampled Data

## Supplementary materials

Timothée Tabouy, Pierre Barbillon and Julien Chiquet

UMR MIA-Paris, AgroParisTech, INRA, Université Paris-Saclay, 75005 Paris,  
France

## Contents

|                                                                            |          |
|----------------------------------------------------------------------------|----------|
| <b>1 Proof of Proposition 1 part (ii)</b>                                  | <b>1</b> |
| <b>2 Identifiability</b>                                                   | <b>1</b> |
| <b>3 Second lower bound in the star degree sampling</b>                    | <b>4</b> |
| <b>4 Proof of Proposition 7</b>                                            | <b>4</b> |
| <b>5 Simulations for star degree and star samplings</b>                    | <b>4</b> |
| <b>6 Additional results for the ER Protein-Protein Interaction network</b> | <b>5</b> |

## 1 Proof of Proposition 1 part (ii)

Recall the following result from graphical model theory (see [Giraud, 2014](#), Formula 7.1).

**Lemma.** *Let  $X, Y, W$  and  $Z$  be random variables, then for all  $h$  measurable,*

$$X \perp\!\!\!\perp (Y, W) \mid Z \Rightarrow X \perp\!\!\!\perp Y \mid (h(W), Z).$$

Applying this lemma with  $h$  the identity function, we get  $R \perp\!\!\!\perp (Y^m, Z) \mid Y^o \Rightarrow R \perp\!\!\!\perp Z \mid (Y^o, Y^m)$ , and then  $R \perp\!\!\!\perp Z \mid (Y^o, Y^m)$  implies  $R \perp\!\!\!\perp Z \mid Y$ .

## 2 Identifiability

When the sampling is node-centered, we denote  $V_i = 1$  if node  $i$  is observed and  $V_i = 0$  otherwise.

*Proof of Proposition 2.* Let  $\rho, \rho' > 0$  be such that  $p_\rho(R) = p_{\rho'}(R)$  (resp.  $p_\rho(V) = p_{\rho'}(V)$ ). Since  $R$  (resp.  $V$ ) does not depend on  $Y$ , then  $\mathbb{P}_\rho(R_{ij} = 1) = \rho = \rho' = \mathbb{P}_{\rho'}(R_{ij} = 1)$  (resp.  $\mathbb{P}_\rho(V_i = 1) = \rho = \rho' = \mathbb{P}_{\rho'}(V_i = 1)$ ).  $\square$

*Proof of Theorem 1.* Let  $P_{[n]}^o$  denote the probability distribution function of  $Y^o$ . We show that there exists a unique  $(\alpha, \pi)$  corresponding to  $P_{[n]}^o$ .

Define  $s_q = \mathbb{P}(Y_{ij}R_{ij} = 1 | Z_{iq} = 1) = \rho(\pi \alpha)_q$  (resp.  $s_q = \mathbb{P}(Y_{ij} = 1 | Z_{iq} = 1) = (\pi \alpha)_q$  for star sampling). Up to reordering,  $s_1 < s_2 < \dots < s_Q$  are the coordinates of the vector

$s$  in the increasing order. Let  $S$  denote the Vandermonde matrix defined by  $S_{i,q} = s_q^i$ , for  $0 \leq i < Q$  and  $1 \leq q \leq Q$ .  $S$  is invertible since the coordinates of  $s$  are all different. For  $i \geq 1$ ,  $S_{i,q} = \mathbb{P}(Y_{12}R_{12} = 1, \dots, Y_{1i+1}R_{1i+1} = 1 | Z_{1q} = 1)$  for random-dyad sampling (resp.  $S_{i,q} = \mathbb{P}(Y_{12} = 1, \dots, Y_{1i+1} = 1 | Z_{1q} = 1)$  for star degree sampling). Let us also define

$$u_i = \sum_{1 \leq k \leq Q} \alpha_k s_k^i \quad (\text{resp. } u_i = \sum_{1 \leq k \leq Q} \rho \alpha_k s_k^i), \quad i = 0, \dots, 2Q-1.$$

For  $i \geq 1$ ,  $u_i = \mathbb{P}(Y_{12}R_{12} = 1, \dots, Y_{1i+1}R_{1i+1} = 1)$  (resp.  $u_i = \mathbb{P}(Y_{12} = 1, \dots, Y_{1i+1} = 1, V_1 = 1)$ ). Note that  $n \geq 2Q$  is a necessary requirement on  $n$  since  $Y_{i,i} = 0$  by assumption. Hence, given  $P_{[n]}^o$  and  $\rho$ ,  $u_0 = 1$  and  $u_1, \dots, u_{2Q-1}$  are known.

Furthermore, set  $M$  the  $(Q+1) \times Q$  matrix given by  $M_{i,j} = u_{i+j}$  for every  $0 \leq i \leq Q$  and  $0 \leq j < Q$ , and let  $M_i$  denote the square matrix obtained by removing the row  $i$  from  $M$ . The coefficients of  $M_Q$ , for  $0 \leq i, j < Q$ , are

$$M_{i,j} = \sum_{1 \leq k \leq Q} s_k^i \alpha_k s_k^j \quad (\text{resp. } M_{i,j} = \sum_{1 \leq k \leq Q} \rho s_k^i \alpha_k s_k^j), \quad \text{with } 0 \leq i, j < Q.$$

Defining the diagonal matrix  $A = \text{Diag}(\alpha)$ , it comes that  $M_Q = SAS^t$  (resp.  $M_Q = \rho SAS^t$ ), where  $S$  and  $A$  are invertible, but unknown at this stage, and  $\rho > 0$ . With  $D_k = \det(M_k)$  and the polynomial  $B(x) = \sum_{k=0}^Q (-1)^{k+Q} D_k x^k$ , it yields  $D_Q = \det(M_Q) \neq 0$  and the degree of  $B$  is equal to  $Q$ .

Set  $C_i = (1, s_i, \dots, s_i^Q)^t$  and let us notice that  $B(s_i)$  is the determinant of the square matrix produced when appending  $C_i$  as the last column to  $M$ . The  $Q+1$  columns of this matrix are linearly dependent, since they are all linear combinations of the  $Q$  vectors  $C_1, C_2, \dots, C_Q$ . Hence  $B(s_i) = 0$  and  $s_i$  is a root of  $B$  for every  $1 \leq i \leq Q$ . This proves that  $B = D_Q \prod_{i=1}^Q (x - s_i)$ . Then, one knows that  $s = (s_1, \dots, s_Q)$  (as the roots of  $B$  defined from  $M$ ) and  $S$ . It results that  $A = S^{-1}M_Q(S^t)^{-1}$ , which yields a unique  $(\alpha_1, \dots, \alpha_Q)$  (resp.  $A = \rho^{-1}S^{-1}M_Q(S^t)^{-1}$ ).

It only remains to determine  $\pi$ . For  $0 \leq i, j < Q$ , let us introduce  $U_{i,j}$  the probability that the first row of  $Y^o$  begins with  $i+1$  occurrences of 1, and the second row of  $Y^o$  ends up with  $j$  occurrences of 1 ( $i+1+j \leq n-1$  implies  $n \geq 2Q$ ). Then,  $U_{i,j} = \sum_{k,l} S_{i,k} \alpha_k \pi_{k,l} \alpha_l S_{j,l}$  (resp.  $U_{i,j} = \sum_{k,l} \rho^2 S_{i,k} \alpha_k \pi_{k,l} \alpha_l S_{j,l}$ ), for  $0 \leq i, j < Q$ , and the  $Q \times Q$  matrix  $U = SA\pi A^t$ . The conclusion results from  $\pi = A^{-1}S^{-1}U(S^t)^{-1}A^{-1}$  (resp.  $\pi = \rho^{-2}A^{-1}S^{-1}U(S^t)^{-1}A^{-1}$ ).  $\square$

*Proof of Theorem 2.* Let  $P_{[n]}$  denote the probability distribution function of  $(Y^o, R)$ . We show that there exists a unique  $(\alpha, \pi, \rho)$  corresponding to  $P_{[n]}$ .

**Identifiability of  $\alpha$ .** Up to reordering, let  $t_1 < t_2 < \dots < t_Q$  denote the coordinates of the vector  $t$  in the increasing order, we have :  $t_q = \mathbb{P}(Y_{ij} = 1, V_j = 1 | Z_{iq} = 1)$ .

Let  $T$  denote the Vandermonde matrix defined by  $T_{i,q} = t_q^i$ , for  $0 \leq i < Q$  and  $1 \leq q \leq Q$ .  $T$  is invertible since the coordinates of  $t$  are all different. For  $i \geq 1$ ,  $T_{i,q} = \mathbb{P}(Y_{12} = 1, \dots, Y_{1i+1} = 1, V_2 = 1, \dots, V_{i+1} = 1 | Z_{1q} = 1)$ . Let us also define

$$v_i = \sum_{1 \leq k \leq Q} \alpha_k t_k^i, \quad i = 0, \dots, 2Q-1.$$

For  $i \geq 1$ ,  $v_i = \mathbb{P}(Y_{12} = 1, \dots, Y_{1i+1} = 1, V_2 = 1, \dots, V_{i+1} = 1)$ . Hence given  $P_{[n]}$ ,  $v_0 = 1$  and  $v_1, \dots, v_{2Q-1}$  are known. Furthermore, set  $N$  the  $(Q+1) \times Q$  matrix given by

$N_{i,j} = v_{i+j}$  for  $0 \leq i \leq j \leq Q$ , and let  $N_i$  denote the square matrix obtained by removing the row  $i$  from  $N$ . The coefficients of  $N_Q$  are

$$N_{i,j} = v_{i+j} = \sum_{1 \leq k \leq Q} t_k^i \alpha_k t_k^j, \quad \text{with } 0 \leq i, j < Q.$$

Defining the diagonal matrix  $A = \text{Diag}(\alpha)$ , it comes that  $N_Q = TAT^t$ , where  $T$  and  $A$  are invertible. With  $D_k = \det(N_k)$  and the polynomial  $B(x) = \sum_{k=0}^Q (-1)^{k+Q} D_k x^k$ , it yields  $D_Q = \det(N_Q) \neq 0$  and the degree of  $B$  is equal to  $Q$ .

Set  $C_i = (1, t_i, \dots, t_i^Q)^t$  and let us notice that  $B(t_i)$  is the determinant of the square matrix produced when appending  $C_i$  as last column to  $N$ . The  $Q+1$  columns of this matrix are linearly dependent, since they are all linear combinations of the  $Q$  vectors  $C_1, C_2, \dots, C_Q$ . Hence  $B(t_i) = 0$  and  $t_i$  is a root of  $B$  for every  $1 \leq i \leq Q$ . This proves that  $B = D_Q \prod_{i=1}^Q (x - t_i)$ . Then, one knows that  $t = (t_1, \dots, t_Q)$  (as the roots of  $B$  defined from  $N$ ) and  $T$ . It results that  $A = T^{-1}N_Q(T^t)^{-1}$ , which yields a unique  $(\alpha_1, \dots, \alpha_Q)$ .

**Identifiability of  $\rho$ .** Up to reordering, let  $o_1 < o_2 < \dots < o_Q$  denote the coordinates of the vector  $o$  in the increasing order, then  $s_q = \mathbb{P}(Y_{ij} = 1, V_i = 1 | Z_{iq} = 1) = \rho_q o_q$ . Let  $O$  denote the Vandermonde matrix defined by  $O_{i,q} = o_q^i$ , for  $0 \leq i < Q$  and  $1 \leq q \leq Q$ .  $O$  is invertible since the coordinates of  $o$  are all different. For  $i \geq 1$ ,  $O_{i,q} = \mathbb{P}(Y_{12} = 1, \dots, Y_{1i+1} = 1 | Z_{1q} = 1)$ . Let us also define

$$u_i = \sum_{1 \leq k \leq Q} \rho_k \alpha_k o_k^i, \quad i = 0, \dots, 2Q-1.$$

For  $i \geq 1$ ,  $u_i = \mathbb{P}(Y_{12} = 1, \dots, Y_{1i+1} = 1, V_1 = 1)$ . Hence given  $P_{[n]}$ ,  $u_0 = 1$  and  $u_1, \dots, u_{2Q-1}$  are known. Furthermore, set  $M$  the  $(Q+1) \times Q$  matrix given by  $M_{i,j} = u_{i+j}$  for every  $0 \leq i \leq Q$  and  $0 \leq j < Q$ , and let  $M_i$  denote the square matrix obtained by removing the row  $i$  from  $M$ . The coefficients of  $M_Q$  are

$$M_{i,j} = u_{i+j} = \sum_{1 \leq k \leq Q} o_k^i \alpha_k \rho_k o_k^j, \quad \text{with } 0 \leq i, j < Q.$$

Defining the diagonal matrix  $B = \text{Diag}(\rho)$ , it comes that  $M_Q = OABO^t$ , where  $O$ ,  $B$  and  $A$  are invertible. Using the same algebraic argument than for the identifiability of  $\alpha$ , it results that  $B = A^{-1}O^{-1}M_Q(O^t)^{-1}$ , which yields, because of the identifiability of  $\alpha$ , a unique  $(\rho_1, \dots, \rho_Q)$ .

**Identifiability of  $\pi$ .** For  $0 \leq i, j < Q$ , let us introduce  $U_{i,j}$  the probability that the first row of  $Y^o$  begins with  $i+1$  occurrences of 1, and the second row of  $Y^o$  ends up with  $j$  occurrences of 1.

$$U_{i,j} = \mathbb{P}\left(\{Y_{12} = 1, \dots, Y_{1i+2} = 1, V_2 = 1, \dots, V_{i+2} = 1\} \cap \{Y_{2n-j} = 1, \dots, Y_{2n} = 1, V_{n-j} = 1, \dots, V_n = 1\}\right),$$

Then,  $U_{i,j} = \sum_{k,l} T_{i,k} \alpha_k \pi_{k,l} \rho_k \alpha_l T_{j,l}$ , for  $0 \leq i, j < Q$ , and the  $Q \times Q$  matrix  $U = TA\pi ABT^t$ . The conclusion results from  $\pi = A^{-1}T^{-1}U(T^t)^{-1}B^{-1}A^{-1}$ . □

### 3 Second lower bound in the star degree sampling

$$\begin{aligned} J_{\tau, \nu, \zeta, \theta, \psi} &= C_{miss} + \sum_{i=1}^n \mathbb{E}_{\tilde{p}} \left[ \text{logistic}(\zeta_i) + \frac{(a + bD_i) - \zeta_i}{2} + h(\zeta_i)((a + bD_i)^2 - \zeta_i^2) \right], \\ &= C_{miss} + \sum_{i=1}^n \left[ \text{logistic}(\zeta_i) + \frac{(a + b\tilde{D}_i) - \zeta_i}{2} + h(\zeta_i)(a^2 + 2ab\tilde{D}_i + b^2\hat{D}_i - \zeta_i^2) \right], \end{aligned}$$

where  $C_{miss} = \sum_{i \in \mathcal{N}^m} (a + b\tilde{D}_i)$  and  $\hat{D}_i = \mathbb{E}_{\tilde{p}} [D_i^2] = \mathbb{V}_{\tilde{p}}(D_i) + \mathbb{E}_{\tilde{p}} [D_i]^2 = \sum_{j \in \mathcal{N}^m} \nu_{ij}(1 - \nu_{ij}) + \left( \sum_{j \in \mathcal{N}^m} \nu_{ij} + \sum_{j \in \mathcal{N}^o} Y_{ij} \right)^2$ .

### 4 Proof of Proposition 7

If the sampling design is node-centered (respectively dyad-centered), the first term in (7) consists in  $n$  Bernoulli random variables (respectively  $n(n-1)/2$  Bernoulli random variables). The term  $\log p_{\psi}(R|Y^o, Y^m, Z, Q)$  can be derived using a BIC approximation:

$$\begin{aligned} \log p_{\psi}(R|Y, Z, Q) &\simeq \arg \max_{\psi} \log p(R|Y, Z, \psi, Q) - \frac{1}{2} \text{pen}_{\text{BIC}}, \\ \text{where } \text{pen}_{\text{BIC}} &= \begin{cases} K \times \log(n) & \text{if the sampling design is node-centered,} \\ K \times \log\left(\frac{n(n-1)}{2}\right) & \text{otherwise.} \end{cases} \end{aligned}$$

### 5 Simulations for star degree and star samplings

With node-centered samplings such as star-degree and class samplings, it is more difficult to find configurations different from MAR sampling designs: with dyad-centred double-standard design, the sampling parameters were directly related to the probability of an edge conditionally on the observation of the corresponding dyad, which is no longer the case for the node-centered designs. The sampling designs being hardly different from a MAR design, the NMAR inference does not show much improvement compared to the MAR inference. Still, we exhibit some interesting situations where star degree and class samplings deserve an appropriate treatment, presented herein. We simulate networks with  $n = 100$  nodes under an affiliation topology with intra-community probability (resp. inter community probability) equal to 0.5 (resp. 0.05) and  $\alpha = (0.25, 0.5, 0.25)$ . Sampling parameters are chosen such that  $\psi = (a, b) = (-3.6, 0.1)$  for star degree sampling, which makes nodes with highest degrees preferably selected. In class sampling, these parameters are set to  $\psi = (\rho_1, \rho_2, \rho_3) = (0.75, 0.5, 0.05)$ , which makes nodes from the largest block and from a small block preferably selected while the other small block is under-sampled. In Figure 1, the estimation errors and the ARI are pictured for both cases. The sampling rates (i.e. rates of observed dyads over total number of dyads) lie in the intervals  $[0.558, 0.844]$  for class sampling and  $[0.162, 0.622]$  for star degree sampling. These two intervals arise from the values of the parameter  $\psi$  explored for these two designs. We compare the performances of Algorithm 2 to an oracle (when inference is conducted via a classical VEM algorithm on a fully observed network) and with Algorithm 1. When facing NMAR condition, Algorithm 2 shows a slight improvement over Algorithm 1 even if it remains far from the oracle.

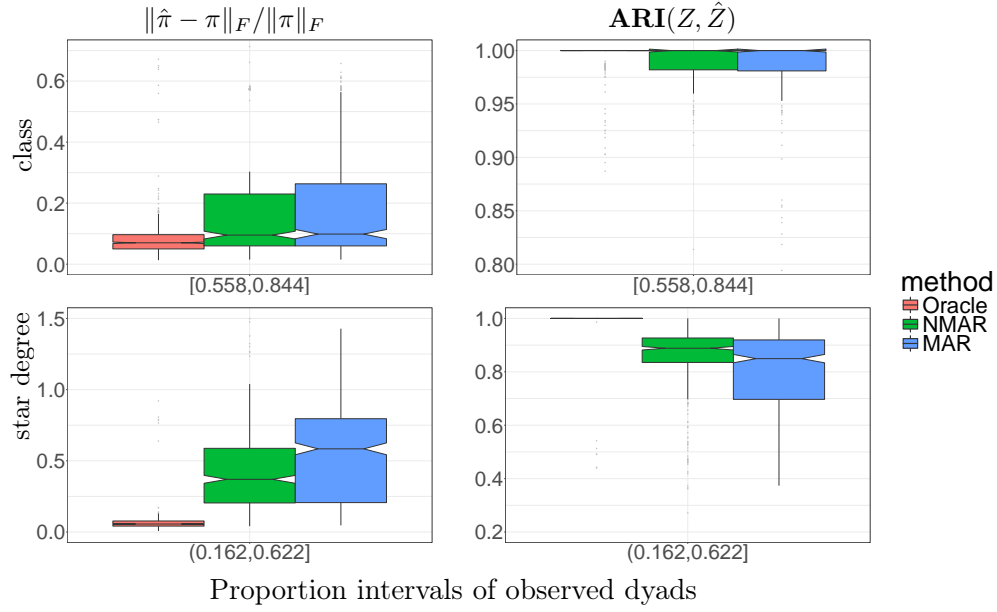

Figure 1: Estimation error of  $\pi$  and ARI averaged over 500 simulations in star degree and class settings. The topology is affiliation with  $\epsilon = 0.05$ .

## 6 Additional results for the ER Protein-Protein Interaction network

In this appendix, we provide more details on the NMAR clustering of the ER network discussed in Section 5.2. We represent the estimated connectivity matrix  $\hat{\pi}$  in Figure 2b for NMAR, which exhibits a network-structure with 13 blocks (or sets of proteins) the sizes of which can be sketched from Figure 2a. In Figure 2c, we represent on the same matrix the network with the original missing data and the imputed missing dyads with the variational parameters  $\nu$ . Interestingly, many of the imputed values are close to 1, which might help validating some relationships which were still uncertain in the biological literature. Figure 2a shows that the MAR clustering leads to a large cluster (block 3) which is mainly split into 4 blocks in the NMAR clustering (blocks 3, 4, 6 and 13).

## References

C. Giraud. Introduction to high-dimensional statistics. Chapman and Hall/CRC, 2014.

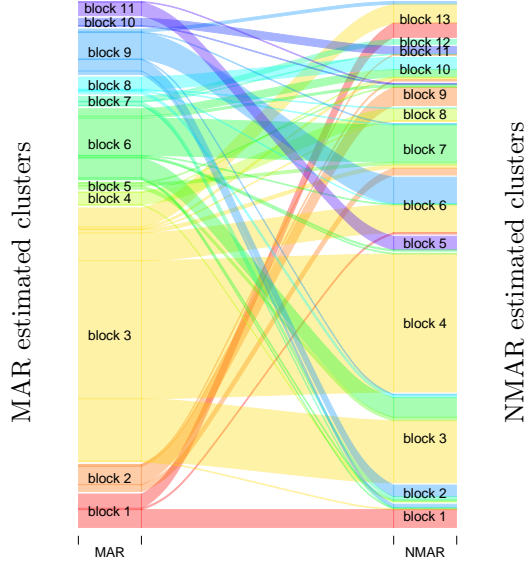

(a) Clustering comparison between MAR and NMAR (11 vs 13 blocks).

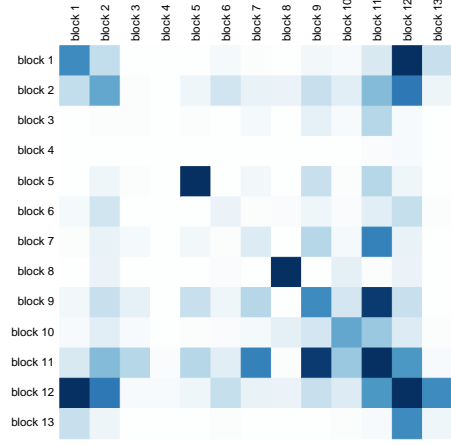

(b) Matrix of connectivity  $\hat{\pi}$  for NMAR inference (double standard) ; intensity of the color is proportional to the probability of connection between blocks.

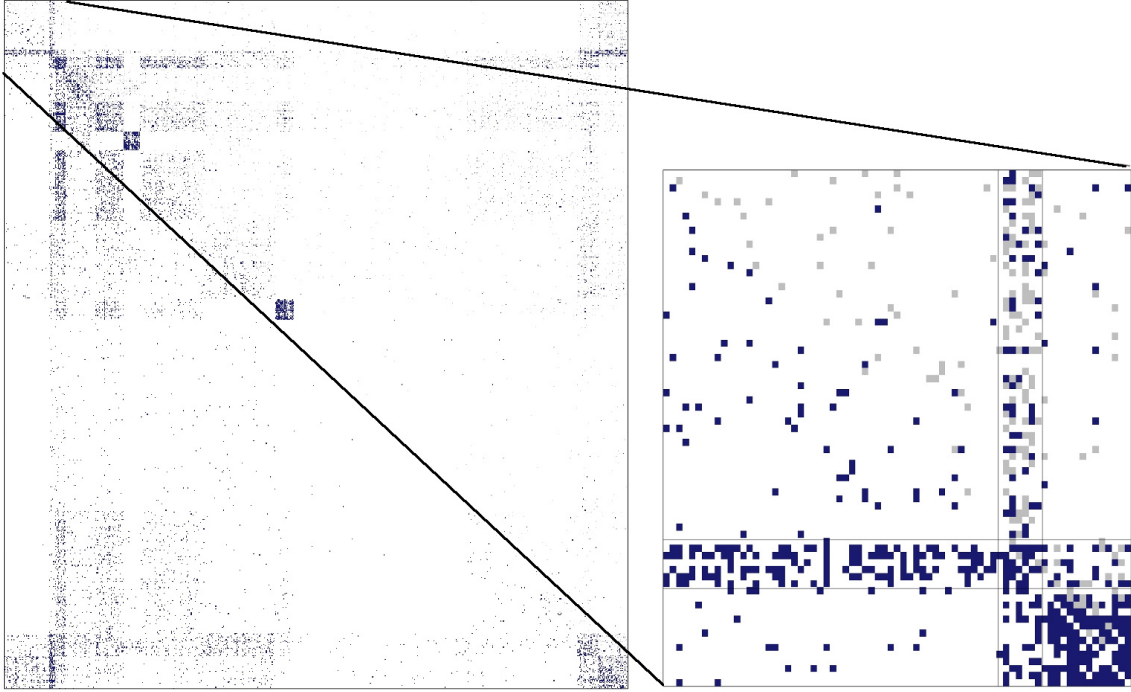

(c) ER PPI network reordered by blocks inferred with SBM with NMAR modeling. Left panel: original data with NA entries colored in gray (upper triangle) and data imputed with  $\nu_{ij}$  (lower triangle); right panel: zoom of blocks (1,2,3).

Figure 2: ER PPI network analysis with SBM under missing data conditions
