# Supplementary material for: Variational Inference for Stochastic Block Models from Sampled Data
Source: arXiv:1707.04141 source file (2019-01-09)
Supplement: Supplementary file 5 [file appendix_proposition_ICL.tex]

\subsection{Proof of Proposition \ref{prop:ICL_NMAR}}

If the sampling design is node-centered (respectively dyad-centered),
the first term in \eqref{eq:complete_loglik_nmar} consists in $n$
Bernoulli random variables (respectively $n(n-1)/2$ Bernoulli random
variables).  The term $\log p_{\psi}(R | \MAO,\MAM, Z, Q)$ can be
derived using a BIC approximation:
\begingroup
\setlength\abovedisplayskip{0pt}
\begin{gather*}\nonumber
\log p_{\psi}(R | \MA, Z, Q) \simeq  {\argmax_{\psi}  } \log p(R | \MA, Z, \psi, Q) - \frac12 \mathrm{pen}_\mathrm{BIC}, \\
 \mathrm{ where } \quad 
  \mathrm{pen}_{\mathrm{BIC}} = \left\{
 \begin{array}{ll}
   K \times \log (n) &  \text{if the sampling design is node-centered,} \\[.2pt]
   K \times \log \left(\frac{n(n-1)}{2}\right) & \text{otherwise.}\\
 \end{array}
 \right.
\end{gather*}
\endgroup
