# Supplementary material for: Variational Inference for Stochastic Block Models from Sampled Data
Source: arXiv:1707.04141 source file (2019-01-09)
Supplement: Supplementary file 6 [file appendix_proposition_mar.tex]

\subsection{Proof of Proposition $\ref{prop:mar}.ii)$}
\label{app:propii}

Recall the following result from graphical model theory
\citep[see][Formula 7.1]{giraud2014}.

\begin{lemma*} Let $X, Y, W$ and $Z$ be random variables, then for all
  $h$ measurable,
  \begin{equation}
    \nonumber
    X \ \indep \ (Y,W) \ | \ Z \Rightarrow \ X \ \indep \ Y \ | \ (h(W), Z).
  \end{equation}
\end{lemma*}  
Applying this lemma with $h$ the identity, function, we get
$R\ \indep \ (\MAM,Z) \ | \ \MAO \Rightarrow \ R \ \indep \ Z \ | \
(\MAO,\MAM)\,$, and then $R \ \indep \ Z \ | \ (\MAO,\MAM)$ implies
$R \ \indep \ Z \ | \ Y$.
