# Supplementary material for: Variational Inference for Stochastic Block Models from Sampled Data
Source: arXiv:1707.04141 source file (2019-01-09)
Supplement: Supplementary file 7 [file appendix_variational.tex]

\subsection{Derivation of second lower bound in star degree sampling}
\label{appendix:variational}

\begin{equation*}
  \begin{aligned}
   J_{\tau,\nu,\zeta,\theta,\psi} & =
     C_{miss} + \sum_{i=1}^n \Ebb_{\tilde{p}}\left[ \text{logistic}(\zeta_i) + \frac{(a+bD_i)-\zeta_i}{2} + h(\zeta_i)((a+bD_i)^2 - \zeta_i^2) \right], \\
    & = C_{miss} + \sum_{i=1}^n \left[ \text{logistic}(\zeta_i) + \frac{(a+b\tilde{D}_i)-\zeta_i}{2} + h(\zeta_i)(a^2 + 2ab\tilde{D}_i + b^{2}\hat{D}_i - \zeta_i^2) \right],
  \end{aligned}
\end{equation*}
where ${C}_{miss} = \sum_{i \in \nodeM} \left( a+b\tilde{D}_i \right)$ and $\hat{D}_i =\Ebb_{\tilde{p}}\left[ {D_i}^2 \right]
= \mathbb{V}_{\tilde{p}}\left( D_i \right) + {\mathbb{E}_{\tilde{p}}\left[ {D_i} \right]}^2 
 =  \sum_{j \in  \nodeM} \nu_{ij}(1-\nu_{ij})  + \left(  \sum_{j \in
     \nodeM} \nu_{ij} + \sum_{j \in \nodeO} \MA_{ij} \right)^2$.

%%% Local Variables:
%%% TeX-master: "TCB_JRSSB_17.tex"
%%% End:
